# Supplementary material for: Astrochemical modelling of infrared dark clouds
Source: arXiv:2111.05379 source file (2022-03-23)
Supplement: Supplementary file 1 [file appendix1.tex]

\begin{appendices}

%\section{The best models found at each position}

%\section{Reaction rates of the models with different Cosmic ray ionization rates}

%\input{chapters/tables/table1_cr}
%\input{chapters/tables/table2_cr}
%\input{chapters/tables/rates-fiducial}
%\input{chapters/tables/table4_cr}
%\input{chapters/tables/table5_cr}
%\input{chapters/tables/table6_cr}

\begin{table*}[ht]
    \centering
    \addtolength{\leftskip} {-2cm}
    \addtolength{\rightskip}{-2cm}
    \begin{tabular}{p{0.26\linewidth}p{0.09\linewidth}p{0.06\linewidth}p{0.07\linewidth}p{0.08\linewidth}p{0.08\linewidth}p{0.1\linewidth}}
    \hline
    \hline
     Fitting & n(H) & T & A$_v$ & $\zeta$ & Time & $\chi^2$\\
     & [cm$^{-3}$] & [K] & [mag] & [s$^{-1}$] & [year] &\\
    \hline
    \rule{0pt}{2ex}
    % Unweighted-unrestricted & 1.0e+04 & 900 & 3 & 1.0e-16 & 1.00e+06 & 1.37e-05\\
    %\rule{0pt}{2ex}
    Weighted-unrestricted & 1.0e+04 & 900 & 3 & 1.0e-16 & 1.00e+06 & 7.34e-04\\
    \hline
    \hline
    Restricted(R) & 2.2e+05 & 15 & 50 & 4.6e-18 & 7.59e+04 & 7.23e-02\\
    (CO,HCO$^+$(O18),N$_2$H$^+$)(Narrow)\\
    (1.0e4-1.0e6[cm$^{-3}$] \\
    (5-100[mag], 5-50[K]) \\
    \rule{0pt}{2ex}
    Ratio (R) & 1.0e+06 & 5 & 50 & 4.6e-16 & 2.24e+05 & 1.82e-05\\
    ions (R) & 1.0e+05 & 10 & 7 & 2.2e-17 & 4.17e+05 & 1.47e-04\\
    CO+ HCO$^+$ & 1.0e+06 & 10 & 50 & 1.0e-15 & 1.95e+04 & 2.38e-03\\
    CO+ N$_2$H$^+$ & 4.6e+05 & 10 & 5 & 2.2e-16 & 6.17e+04 & 1.89e-03\\
    \rule{0pt}{5ex}
    R+ CH$_3$OH,H$_2$CO & 2.2e+05 & 25 & 5 & 2.2e-19 & 1.00e+08 & 3.92e+00\\
    R+ H$_2$CO & 2.2e+04 & 20 & 5 & 1.0e-19 & 2.00e+07 & 6.45e-01\\
    R+ HNCO,HNC,HCN & 1.0e+06 & 10 & 100 & 1.0e-15 & 1.20e+04 & 6.26e+00\\
    R + N-group + C-group & 1.0e+06 & 30 & 50 & 4.6e-18 & 9.12e+07 & 1.46e+01\\
    R+ N-group + H$_2$CO & 1.0e+06 & 30 & 50 & 4.6e-18 & 9.12e+07 & 1.50e+01\\
    \hline
    \end{tabular}
    \vspace*{2mm}
    \caption{The best models found with different solutions at p1. The restricted fitting have been performed through the models with Hnuc in the range of 1.0e4-1.0e6 cm-3, temperature in the range of 5-50 K and and visual extinction in the range of 5-100 mag.}
    \label{tab:p1_different_fittings}
\end{table*}
\begin{table*}[ht]
    \centering
    \addtolength{\leftskip} {-2cm}
    \addtolength{\rightskip}{-2cm}
    \begin{tabular}{p{0.26\linewidth}p{0.09\linewidth}p{0.06\linewidth}p{0.07\linewidth}p{0.08\linewidth}p{0.08\linewidth}p{0.1\linewidth}}
    \hline
    \hline
     Fitting & n(H) & T & A$_v$ & $\zeta$ & Time & $\chi^2$\\
     & [cm$^{-3}$] & [K] & [mag] & [s$^{-1}$] & [year] &\\
    \hline
    \hline
    Restricted & 1.0e+04 & 15 & 100 & 2.2e-19 & 2.29e+06 & 5.72e-02\\
    (CO,HCO$^+$(O18),N$_2$H$^+$)(Narrow)\\
    (1.0e4-1.0e6[cm$^{-3}$] \\
    (5-100[mag], 5-50[K]) \\
    \rule{0pt}{2ex}
    Ratio (R) & 1.0e+04 & 15 & 20 & 4.6e-19 & 1.86e+06 & 6.73e-04\\
    ions (R) & 4.6e+04 & 15 & 10 & 4.6e-19 & 6.92e+07 & 3.49e-03\\
    CO+ HCO$^+$ & 2.2e+04 & 10 & 5 & 1.0e-18 & 9.77e+05 & 3.11e-03\\
    CO+ N$_2$H$^+$ & 4.6e+05 & 25 & 10 & 1.0e-17 & 1.82e+07 & 6.18e-04\\
    \rule{0pt}{5ex}
     R+ CH$_3$OH,H$_2$CO & 1.0e+04 & 20 & 5 & 2.2e-19 & 3.63e+07 & 1.26e+01\\
    R+ H$_2$CO & 1.0e+04 & 20 & 5 & 1.0e-19 & 2.24e+07 & 9.15e-01\\
    R+ HNCO,HNC,HCN & 1.0e+06 & 10 & 100 & 2.2e-15 & 1.02e+04 & 1.49e+01\\
    R+ N-group + C-group & 1.0e+06 & 30 & 50 & 4.6e-18 & 1.00e+08 & 2.27e+01 \\
    R+ N-group + H$_2$CO & 1.0e+06 & 30 & 50 & 4.6e-18 & 1.00e+08 & 1.80e+01\\
    \hline
    \end{tabular}
    \vspace*{2mm}
    \caption{The best models found with different solutions at p2. The restricted fitting have been performed through the models with Hnuc in the range of 1.0e4-1.0e6 cm-3, temperature in the range of 5-50 K and and visual extinction in the range of 5-100 mag}
    \label{tab:p2_different_fittings}
\end{table*}
\begin{table*}[ht]
    \centering
    \addtolength{\leftskip} {-2cm}
    \addtolength{\rightskip}{-2cm}
    \begin{tabular}{p{0.26\linewidth}p{0.09\linewidth}p{0.06\linewidth}p{0.07\linewidth}p{0.08\linewidth}p{0.08\linewidth}p{0.1\linewidth}}
    \hline
    \hline
     Fitting & n(H) & T & A$_v$ & $\zeta$ & Time & $\chi^2$\\
     & [cm$^{-3}$] & [K] & [mag] & [s$^{-1}$] & [year] &\\
    \hline
    \rule{0pt}{2ex}
     %Unweighted-unrestricted & 2.2e+06 & 500 & 2 & 2.2e-14 & 1.58e+04 & 5.64e-04\\
    %\rule{0pt}{2ex}
    Weighted-unrestricted & 2.2e+06 & 500 & 2 & 2.2e-14 & 1.55e+04 & 3.24e-02 \\
    %\rule{0pt}{2ex}
    %Unweighted-restricted & 1.0e+04 & 15 & 20 & 2.2e-19 & 1.91e+06 & 7.83e-03 \\
    \hline
    \hline
    Restricted & 1.0e+04 & 15 & 50 & 2.2e-19 & 2.04e+06 & 5.68e-02\\
    (CO,HCO$^+$(O18),N$_2$H$^+$)(Narrow)\\
    (1.0e4-1.0e6[cm$^{-3}$] \\
    (5-100[mag], 5-50[K]) \\
    \rule{0pt}{2ex}
    Ratio (R) & 1.0e+04 & 15 & 20 & 4.6e-19 & 1.70e+06 & 1.81e-04\\
    ions (R) & 1.0e+06 & 5 & 7 & 1.0e-13 & 1.91e+04 & 7.74e-04\\
    CO+ HCO$^+$ & 2.2e+04 & 10 & 5 & 1.0e-18 & 9.12e+05 & 1.55e-03\\
    CO+ N$_2$H$^+$ & 1.0e+04 & 15 & 5 & 2.2e-19 & 2.04e+06 & 3.63e-04\\
    \rule{0pt}{5ex}
    R+ CH$_3$OH,H$_2$CO & 1.0e+05 & 25 & 5 & 2.2e-19 & 1.00e+08 & 1.33e+01\\
    R+ H$_2$CO & 1.0e+04 & 20 & 5 & 1.0e-19 & 2.19e+07 & 7.53e-01\\
    R+ HNCO,HNC,HCN & 1.0e+06 & 10 & 100 & 2.2e-15 & 1.05e+04 & 1.65e+01\\
    R + N-group + C-group & 1.0e+06 & 30 & 50 & 4.6e-18 & 1.00e+08 & 2.64e+01 \\
    R+ N-group + H$_2$CO & 1.0e+04 & 30 & 100 & 1.0e-18 & 2.19e+07 & 2.09e+01\\
    \hline
    \end{tabular}
    \vspace*{2mm}
    \caption{The best models found with different solutions at p3. The restricted fitting have been performed through the models with Hnuc in the range of 1.0e4-1.0e6 cm-3, temperature in the range of 5-50 K and and visual extinction in the range of 5-100 mag.}
    \label{tab:p3_different_fittings}
\end{table*}
\begin{table*}[ht]
    \centering
    \addtolength{\leftskip} {-2cm}
    \addtolength{\rightskip}{-2cm}
    \begin{tabular}{p{0.26\linewidth}p{0.09\linewidth}p{0.06\linewidth}p{0.07\linewidth}p{0.08\linewidth}p{0.08\linewidth}p{0.1\linewidth}}
    \hline
    \hline
     Fitting & n(H) & T & A$_v$ & $\zeta$ & Time & $\chi^2$\\
     & [cm$^{-3}$] & [K] & [mag] & [s$^{-1}$] & [year] &\\
    \hline
    \rule{0pt}{2ex}
     %Unweighted-unrestricted & 1.0e+07 & 500 & 1 & 1.0e-13 & 6.03e+04 & 7.19e-04\\
    %\rule{0pt}{2ex}
    Weighted-unrestricted & 2.2e+06 & 500 & 2 & 2.2e-14 & 1.17e+04 & 3.89e-02 \\
    %\rule{0pt}{2ex}
    %unweighted-restricted & 1.0e+04 & 15 & 20 & 2.2e-19 & 1.86e+06 & 6.03e-03 \\
    \hline
    \hline
    Restricted & 1.0e+04 & 15 & 7 & 2.2e-19 & 2.04e+06 & 1.17e-03\\
    (CO,HCO$^+$(O18),N$_2$H$^+$)(Narrow)\\
    (1.0e4-1.0e6[cm$^{-3}$] \\
    (5-100[mag], 5-50[K]) \\
    \rule{0pt}{2ex}
    Ratio (R) & 4.6e+05 & 15 & 5 & 2.2e-19 & 6.76e+04 & 1.39e-05\\
    ions (R) & 1.0e+05 & 5 & 10 & 1.0e-14 & 2.00e+05 & 7.86e-05\\
    CO+ HCO$^+$ & 1.0e+04 & 15 & 7 & 2.2e-19 & 2.04e+06 & 6.81e-04\\
    CO+ N$_2$H$^+$ & 1.0e+06 & 10 & 5 & 4.6e-15 & 2.88e+04 & 1.72e-06\\
    \rule{0pt}{5ex}
     R+ CH$_3$OH,H$_2$CO & 1.0e+05 & 25 & 5 & 2.2e-19 & 1.00e+08 & 1.16e+01\\
    R+ H$_2$CO & 1.0e+04 & 20 & 5 & 1.0e-19 & 2.19e+07 & 6.02e-01\\
    R+ HNCO,HNC,HCN & 1.0e+06 & 10 & 100 & 2.2e-15 & 1.05e+04 & 1.39e+01\\
    R+ N-group + C-group & 1.0e+06 & 30 & 50 & 4.6e-18 & 1.00e+08 & 2.17e+01 \\
    R+ N-group + H$_2$CO & 1.0e+04 & 30 & 20 & 1.0e-18 & 2.19e+07 & 1.85e+01\\
    \hline
    \end{tabular}
    \vspace*{2mm}
    \caption{The best models found with different solutions at p4. The restricted fitting have been performed through the models with Hnuc in the range of 1.0e4-1.0e6 cm-3, temperature in the range of 5-50 K and and visual extinction in the range of 5-100 mag.}
    \label{tab:p4_different_fittings}
\end{table*}
\begin{table*}[ht]
    \centering
    \addtolength{\leftskip} {-2cm}
    \addtolength{\rightskip}{-2cm}
    \begin{tabular}{p{0.26\linewidth}p{0.09\linewidth}p{0.06\linewidth}p{0.07\linewidth}p{0.08\linewidth}p{0.08\linewidth}p{0.1\linewidth}}
    \hline
    \hline
     Fitting & n(H) & T & A$_v$ & $\zeta$ & Time & $\chi^2$\\
     & [cm$^{-3}$] & [K] & [mag] & [s$^{-1}$] & [year] &\\
    \hline
    \rule{0pt}{2ex}
     %Unweighted-unrestricted & 4.6e+03 & 500 & 5 & 4.6e-17 & 1.15e+07 & 1.15e-04\\
    %\rule{0pt}{2ex}
    Weighted-unrestricted & 4.6e+03 & 500 & 5 & 4.6e-17 & 1.17e+07 & 6.18e-03 \\
    %\rule{0pt}{2ex}
    %Unweighted-restricted & 2.2e+04 & 15 & 20 & 4.6e-19 & 7.24e+05 & 5.64e-03 \\
    \hline
    \hline
    Restricted & 1.0e+05 & 15 & 5 & 4.6e-18 & 1.48e+05 & 8.12e-02\\
    (CO,HCO$^+$(O18),N$_2$H$^+$)(Narrow)\\
    (1.0e4-1.0e6[cm$^{-3}$] \\
    (5-100[mag], 5-50[K]) \\
    \rule{0pt}{2ex}
    Ratio (R) & 1.0e+06 & 5 & 50 & 2.2e-16 & 1.86e+05 & 2.79e-03\\
    ions (R) & 4.6e+05 & 25 & 50 & 4.6e-17 & 6.03e+06 & 1.56e-03\\
    CO+ HCO$^+$ & 4.6e+04 & 10 & 10 & 2.2e-18 & 3.98e+05 & 1.81e-03\\
    CO+ N$_2$H$^+$ & 1.0e+06 & 10 & 7 & 2.2e-15 & 2.75e+04 & 1.25e-03\\
    \rule{0pt}{5ex}
    R+ CH$_3$OH,H$_2$CO & 1.0e+05 & 25 & 5 & 2.2e-19 & 1.00e+08 & 8.93e+00\\
    R+ H$_2$CO & 1.0e+04 & 20 & 5 & 1.0e-19 & 2.14e+07 & 7.53e-01\\
    R+ HNCO,HNC,HCN & 1.0e+06 & 10 & 100 & 1.0e-15 & 1.15e+04 & 1.14e+01\\
    R+ N-group + C-group & 1.0e+06 & 30 & 50 & 4.6e-18 & 1.00e+08 & 1.88e+01\\
    R+ N-group + H$_2$CO & 1.0e+04 & 30 & 100 & 1.0e-18 & 2.19e+07 & 1.54e+01\\
    \hline
    \end{tabular}
    \vspace*{2mm}
    \caption{The best models found with different solutions at p5. The restricted fitting have been performed through the models with Hnuc in the range of 1.0e4-1.0e6 cm-3, temperature in the range of 5-50 K and and visual extinction in the range of 5-100 mag.}
    \label{tab:p5_different_fittings}
\end{table*}
\begin{table*}[ht]
    \centering
    \addtolength{\leftskip} {-2cm}
    \addtolength{\rightskip}{-2cm}
    \begin{tabular}{p{0.26\linewidth}p{0.09\linewidth}p{0.06\linewidth}p{0.07\linewidth}p{0.08\linewidth}p{0.08\linewidth}p{0.1\linewidth}}
    \hline
    \hline
     Fitting & n(H) & T & A$_v$ & $\zeta$ & Time & $\chi^2$\\
     & [cm$^{-3}$] & [K] & [mag] & [$s^{-1}$] & [year] &\\
    \hline
    \rule{0pt}{2ex}
     %Unweighted-unrestricted & 2.2e+03 & 450 & 7 & 2.2e-17 & 6.46e+06 & 5.86e-04\\
    %\rule{0pt}{2ex}
    Weighted-unrestricted & 2.2e+03 & 450 & 7 & 2.2e-17 & 6.46e+06 & 3.15e-02\\
    %\rule{0pt}{2ex}
    %Unweighted-restricted & 1.0e+04 & 15 & 20 & 1.0e-18 & 1.15e+06 & 3.55e-02 \\
    \hline
    \hline
    Restricted & 1.0e+04 & 5 & 7 & 1.0e-15 & 2.04e+06 & 2.01e+00\\
    (CO,HCO$^+$(O18),N$_2$H$^+$)(Narrow) & 1.0e+04 & 15 & 5 & 4.6e-19 & 1.66e+06 & 2.35e+00\\
    (1.0e4-1.0e6[cm$^{-3}$] \\
    (5-100[mag], 5-50[K]) \\
    \rule{0pt}{2ex}
    Ratio (R) & 2.2e+04 & 5 & 100 & 1.0e-18 & 2.45e+07 & 1.85e-03\\
    ions (R) & 1.0e+05 & 15 & 5 & 2.2e-17 & 5.50e+06 & 2.05e-03\\
    CO+ HCO$^+$ & 2.2e+05 & 10 & 7 & 4.6e-18 & 5.75e+04 & 9.52e-06\\
    CO+ N$_2$H$^+$ & 4.6e+05 & 10 & 7 & 2.2e-15 & 4.17e+04 & 1.94e-03\\
    \rule{0pt}{5ex}
    R+ CH$_3$OH,H$_2$CO & 1.0e+04 & 20 & 5 & 2.2e-19 & 2.82e+07 & 1.65e+01\\
    R+ H$_2$CO & 1.0e+04 & 20 & 5 & 1.0e-19 & 2.19e+07 & 7.28e+00\\
    R+ HNCO,HNC,HCN & 1.0e+06 & 10 & 100 & 4.6e-15 & 9.33e+03 & 8.23e+00\\
    R+ N-group + C-group & 1.0e+06 & 30 & 50 & 4.6e-18 & 1.00e+08 & 1.79e+01\\
    R+ N-group + H$_2$CO & 1.0e+04 & 30 & 10 & 1.0e-18 & 1.91e+07 & 1.87e+01\\
    \hline
    \end{tabular}
    \vspace*{2mm}
    \caption{The best models found with different solutions at p6. The restricted fitting have been performed through the models with n(H) in the range of 1.0e4-1.0e6 cm-3, temperature in the range of 5-50 K and and visual extinction in the range of 5-100 mag.}
    \label{tab:p6_different_fittings}
\end{table*}
\begin{table*}[ht]
    \centering
    \addtolength{\leftskip} {-2cm}
    \addtolength{\rightskip}{-2cm}
    \begin{tabular}{p{0.26\linewidth}p{0.09\linewidth}p{0.06\linewidth}p{0.07\linewidth}p{0.08\linewidth}p{0.08\linewidth}p{0.1\linewidth}}
    \hline
    \hline
     Fitting & n(H) & T & A$_v$ & $\zeta$ & Time & $\chi^2$\\
     & [cm$^{-3}$] & [K] & [mag] & [s$^{-1}$] & [year] &\\
    \hline
    \rule{0pt}{2ex}
     %Unweighted-unrestricted & 4.6e+04 & 15 & 2 & 1.0e-17 & 1.00e+08 & 1.43e-03\\
    %\rule{0pt}{2ex}
    Weighted-unrestricted & 2.2e+03 & 600 & 5 & 2.2e-17 & 7.59e+06 & 7.79e-02 \\
    %\rule{0pt}{2ex}
    %Unweighted-restricted & 1.0e+04 & 15 & 20 & 2.2e-19 & 1.45e+06 & 5.31e-03\\
    \hline
    \hline
    Restricted & 2.2e+04 & 15 & 5 & 4.6e-19 & 6.92e+05 & 6.78e-02\\
    (CO,HCO$^+$(O18),N$_2$H$^+$)(Narrow)\\
    (1.0e4-1.0e6[cm$^{-3}$] \\
    (5-100[mag], 5-50[K]) \\
    \rule{0pt}{2ex}
    Ratio (R) & 4.6e+04 & 10 & 5 & 1.0e-19 & 1.07e+06 & 1.70e-03\\
    ions (R) & 1.0e+05 & 15 & 7 & 4.6e-18 & 1.15e+07 & 8.36e-05\\
    CO+ HCO$^+$ & 1.0e+04 & 25 & 7 & 2.2e-14 & 3.98e+03 & 5.31e-05\\
    CO+ N$_2$H$^+$ & 4.6e+04 & 10 & 5 & 1.0e-17 & 3.63e+05 & 6.45e-04\\
    \rule{0pt}{5ex}
     R+ CH$_3$OH,H$_2$CO & 2.2e+05 & 25 & 5 & 2.2e-19 & 1.00e+08 & 7.23e+00\\
    R+ H$_2$CO & 2.2e+04 & 20 & 5 & 1.0e-19 & 2.04e+07 & 1.81e+00\\
    R+ HNCO,HNC,HCN & 1.0e+06 & 10 & 100 & 1.0e-15 & 1.20e+04 & 9.02e+00\\
    R+ N-group + C-group & 1.0e+06 & 30 & 20 & 4.6e-18 & 9.33e+07 & 1.72e+01\\
    R+ N-group + H$_2$CO & 1.0e+04 & 30 & 10 & 4.6e-19 & 3.47e+07 & 1.82e+01\\
    \hline
    \end{tabular}
    \vspace*{2mm}
    \caption{The best models found with different solutions at p7. The restricted fitting have been performed through the models with Hnuc in the range of 1.0e4-1.0e6 cm-3, temperature in the range of 5-50 K and and visual extinction in the range of 5-100 mag.}
    \label{tab:p7_different_fittings}
\end{table*}
\begin{table*}[ht]
    \centering
    \addtolength{\leftskip} {-2cm}
    \addtolength{\rightskip}{-2cm}
    \begin{tabular}{p{0.26\linewidth}p{0.09\linewidth}p{0.06\linewidth}p{0.07\linewidth}p{0.08\linewidth}p{0.08\linewidth}p{0.1\linewidth}}
    \hline
    \hline
     Fitting & n(H) & T & A$_v$ & $\zeta$ & Time & $\chi^2$\\
     & [cm$^{-3}$] & [K] & [mag] & [s$^{-1}$] & [year] &\\
    \hline
    \rule{0pt}{2ex}
     %Unweighted-unrestricted & 4.6e+04 & 15 & 2 & 2.2e-19 & 2.88e+05 & 1.13e-04 \\
    %\rule{0pt}{2ex}
    Weighted-unrestricted & 4.6e+04 & 15 & 2 & 2.2e-19 & 2.88e+05 & 5.80e-03 \\
    %\rule{0pt}{2ex}
    %Unweighted-restricted & 1.0e+04 & 15 & 100 & 1.0e-19 & 1.78e+06 & 4.16e-03 \\
    \hline
    \hline
    Restricted & 1.0e+04 & 20 & 5 & 1.0e-19 & 2.04e+07 & 2.95e-02\\
    (CO,HCO$^+$(O18),N$_2$H$^+$)(Narrow)\\
    (1.0e4-1.0e6[cm$^{-3}$] \\
    (5-100[mag], 5-50[K]) \\
    \rule{0pt}{2ex}
    Ratio (R) & 2.2e+04 & 5 & 100 & 1.0e-18 & 1.95e+07 & 7.62e-04\\
    ions (R) & 1.0e+05 & 15 & 5 & 1.0e-17 & 1.55e+07 & 2.14e-04\\
    CO+ HCO$^+$ & 1.0e+06 & 10 & 50 & 4.6e-16 & 1.82e+04 & 1.49e-03\\
    CO+ N$_2$H$^+$ & 1.0e+06 & 10 & 100 & 2.2e-15 & 1.74e+04 & 7.43e-05\\
    \rule{0pt}{5ex}
     R+ CH$_3$OH,H$_2$CO & 2.2e+05 & 25 & 5 & 2.2e-19 & 2.88e+07 & 6.06e+00\\
    R+ H$_2$CO & 4.6e+04 & 20 & 5 & 1.0e-19 & 2.09e+07 & 1.89e+00\\
    R+ HNCO,HNC,HCN & 1.0e+06 & 10 & 100 & 1.0e-15 & 1.35e+04 & 8.33e+00\\
    R+ N-group + C-group & 1.0e+06 & 30 & 50 & 4.6e-18 & 9.12e+07 & 1.67e+01\\
    R+ N-group + H$_2$CO & 1.0e+04 & 30 & 10 & 4.6e-19 & 3.47e+07 & 1.78e+01\\
    \hline
    \end{tabular}
    \vspace*{2mm}
    \caption{The best models found with different solutions at p8. The restricted fitting have been performed through the models with Hnuc in the range of 1.0e4-1.0e6 cm-3, temperature in the range of 5-50 K and and visual extinction in the range of 5-100 mag.}
    \label{tab:p8_different_fittings}
\end{table*}
\begin{table*}[ht]
    \centering
    \addtolength{\leftskip} {-2cm}
    \addtolength{\rightskip}{-2cm}
    \begin{tabular}{p{0.26\linewidth}p{0.09\linewidth}p{0.06\linewidth}p{0.07\linewidth}p{0.08\linewidth}p{0.08\linewidth}p{0.1\linewidth}}
    \hline
    \hline
     Fitting & n(H) & T & A$_v$ & $\zeta$ & Time & $\chi^2$\\
     & [cm$^{-3}$] & [K] & [mag] & [s$^{-1}$] & [year] &\\
    \hline
    \rule{0pt}{2ex}
     %Unweighted-unrestricted & 2.2e+04 & 500 & 4 & 2.2e-16 & 3.02e+06 & 2.04e-04\\
    %\rule{0pt}{2ex}
    Weighted-unrestricted & 2.2e+04 & 500 & 4 & 2.2e-16 & 3.16e+06 & 1.16e-02 \\
    %\rule{0pt}{2ex}
    %Unweighted-restricted & 1.0e+04 & 15 & 20 & 2.2e-19 & 1.66e+06 & 4.94e-03\\
    \hline
    \hline
    Restricted & 4.6e+04 & 15 & 5 & 1.0e-18 & 3.63e+05 & 4.63e-02\\
    (CO,HCO$^+$(O18),N$_2$H$^+$)(Narrow)\\
    (1.0e4-1.0e6[cm$^{-3}$] \\
    (5-100[mag], 5-50[K]) \\
     \rule{0pt}{2ex}
    Ratio (R) & 1.0e+04 & 15 & 5 & 1.0e-19 & 2.24e+06 & 1.52e-03\\
    ions (R) & 4.6e+05 & 5 & 20 & 1.0e-13 & 3.89e+04 & 5.75e-04\\
    CO+ HCO$^+$ & 1.0e+04 & 20 & 20 & 2.2e-14 & 5.01e+03 & 1.49e-04\\
    CO+ N$_2$H$^+$ & 4.6e+05 & 10 & 20 & 2.2e-16 & 4.37e+04 & 1.01e-03\\
    \rule{0pt}{5ex}
    R+ CH$_3$OH,H$_2$CO & 1.0e+05 & 25 & 5 & 2.2e-19 & 3.72e+07 & 1.00e+01\\
    R+ H$_2$CO & 1.0e+04 & 20 & 5 & 1.0e-19 & 2.14e+07 & 1.31e-01\\
    R+ HNCO,HNC,HCN & 1.0e+06 & 10 & 100 & 1.0e-15 & 1.17e+04 & 1.36e+01\\
    R+ N-group + C-group & 1.0e+06 & 30 & 50 & 4.6e-18 & 1.00e+08 & 2.19e+01\\
    R+ N-group + H$_2$CO & 1.0e+06 & 30 & 50 & 4.6e-18 & 1.00e+08 & 1.79e+01\\
    \hline
    \end{tabular}
    \vspace*{2mm}
    \caption{The best models found with different solutions at p9. The restricted fitting have been performed through the models with Hnuc in the range of 1.0e4-1.0e6 cm-3, temperature in the range of 5-50 K and and visual extinction in the range of 5-100 mag.}
    \label{tab:p9_different_fittings}
\end{table*}
\begin{table*}[ht]
    \centering
    \addtolength{\leftskip} {-2cm}
    \addtolength{\rightskip}{-2cm}
    \begin{tabular}{p{0.26\linewidth}p{0.09\linewidth}p{0.06\linewidth}p{0.07\linewidth}p{0.08\linewidth}p{0.08\linewidth}p{0.1\linewidth}}
    \hline
    \hline
     Fitting & n(H) & T & A$_v$ & $\zeta$ & Time & $\chi^2$\\
     & [cm$^{-3}$] & [K] & [mag] & [s$^{-1}$] & [year] &\\
    \hline
    \rule{0pt}{2ex}
     %Unweighted-unrestricted & 1.0e+07 & 600 & 1 & 1.0e-13 & 1.23e+03 & 8.65e-05\\
    %\rule{0pt}{2ex}
    Weighted-unrestricted & 1.0e+07 & 600 & 1 & 1.0e-13 & 1.23e+03 & 4.69e-03 \\
    %\rule{0pt}{2ex}
    %Unweighted-restricted & 1.0e+04 & 15 & 20 & 4.6e-19 & 1.35e+06 & 1.13e-02 \\
    \hline
    \hline
    Restricted & 1.0e+04 & 15 & 5 & 2.2e-19 & 1.86e+06 & 1.23e-01\\
    (CO,HCO$^+$(O18),N$_2$H$^+$)(Narrow)\\
    (1.0e4-1.0e6[cm$^{-3}$] \\
    (5-100[mag], 5-50[K]) \\
    \rule{0pt}{2ex}
    Ratio (R) & 2.2e+05 & 15 & 5 & 4.6e-19 & 1.15e+05 & 4.40e-04\\
    ions (R) & 1.0e+04 & 15 & 5 & 2.2e-19 & 2.00e+06 & 1.31e-04\\
    CO+ HCO$^+$ & 2.2e+04 & 25 & 100 & 4.6e-14 & 1.86e+03 & 5.70e-04\\
    CO+ N$_2$H$^+$ & 4.6e+04 & 15 & 5 & 2.2e-18 & 3.16e+05 & 2.83e-04\\
    \rule{0pt}{5ex}
     R+ CH$_3$OH,H$_2$CO & 1.0e+05 & 25 & 5 & 2.2e-19 & 1.00e+08 & 1.32e+01\\
    R+ H$_2$CO & 1.0e+04 & 20 & 5 & 1.0e-19 & 2.19e+07 & 8.12e-01\\
    R+ HNCO,HNC,HCN & 1.0e+06 & 10 & 100 & 2.2e-15 & 1.05e+04 & 1.25e+01\\
    R+ N-group + C-group & 1.0e+06 & 30 & 50 & 4.6e-18 & 1.00e+08 & 2.30e+01\\
    R+ N-group + H$_2$CO & 1.0e+06 & 10 & 100 & 2.2e-15 & 1.07e+04 & 1.67e+01\\
    \hline
    \end{tabular}
    \vspace*{2mm}
    \caption{The best models found with different solutions at p10. The restricted fitting have been performed through the models with Hnuc in the range of 1.0e4-1.0e6 cm-3, temperature in the range of 5-50 K and and visual extinction in the range of 5-100 mag.}
    \label{tab:p10_different_fittings}
\end{table*}

\end{appendices}
