# Supplementary material for: Astrochemical modelling of infrared dark clouds
Source: arXiv:2111.05379 source file (2022-03-23)
Supplement: Supplementary file 2 [file appendix4.tex]

\begin{appendices}
%%%%%%%%%%%%%%%%%%%%%%%%%%%%%%%%%%%%%%%55
\begin{figure*}[!ht]
   \centering
     %\addtolength{\leftskip} {-8cm}
    %\addtolength{\rightskip}{-8.5cm}
     \includegraphics[width=\textwidth]{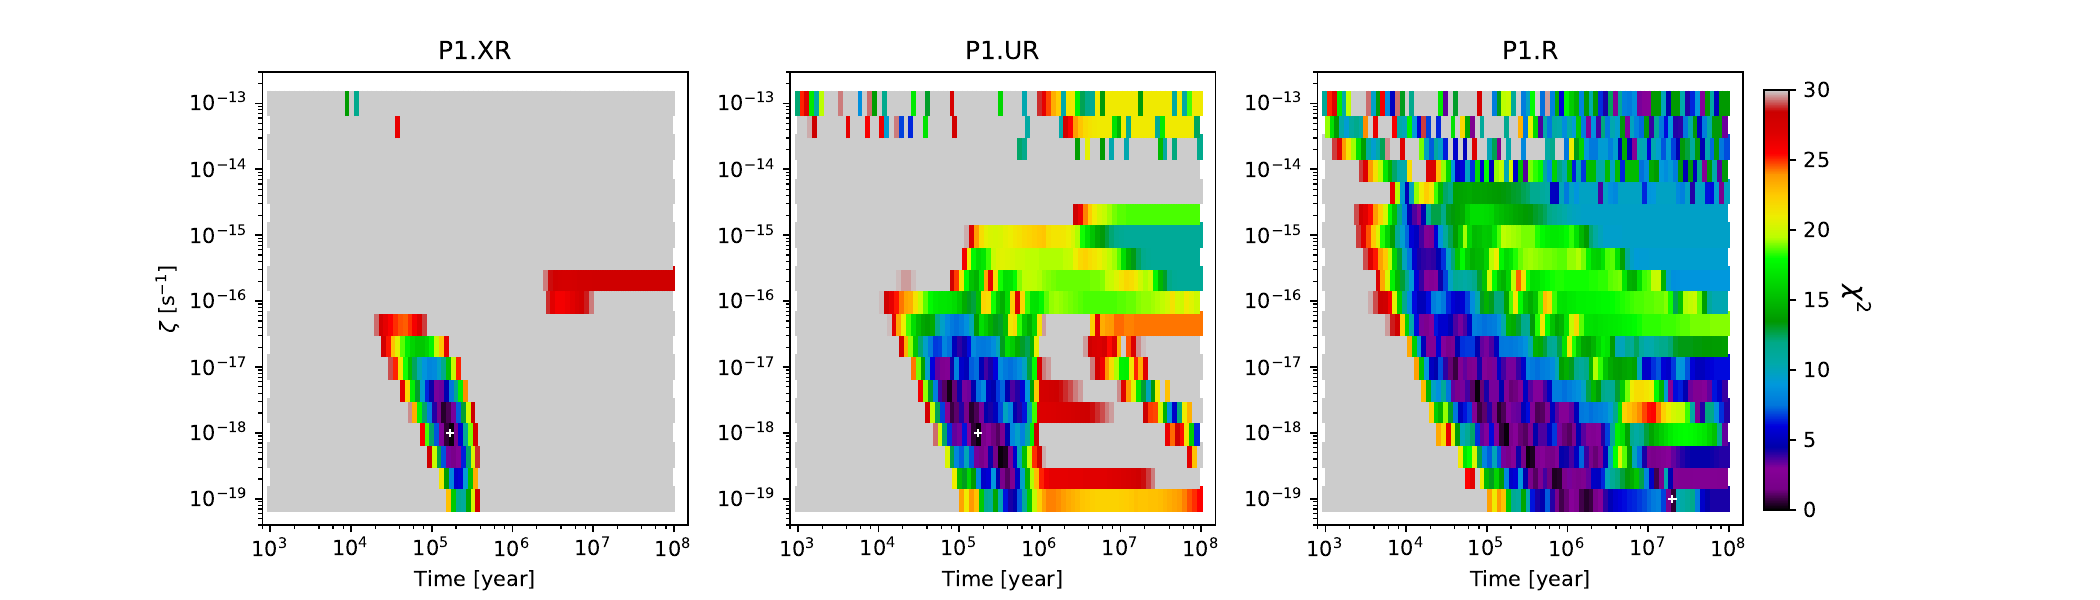}
     %\vspace{0.01cm}
     \caption{\tiny Distribution of $\zeta$ associated with $\chi^2$ using abundances of three main species CO, HCO$^+$ and N$_2$H$^+$ at P1, XR) Extra-Restricted area at which n$_H$ = 1.0e5 cm$^{-3}$, T=15 K and A$_v$=20 mag are held to be fixes and $\zeta$ has been changed, UR) Ultra-Restricted area at which n$_H$=4.6e4,1.0e5,2.2e5 cm$^{-3}$, T=10,15,20 K and A$_v$=10,20,50 mag, R) Restricted area at which n$_H$=1.0e4e4-1.0e6 cm$^{-3}$, T=10-50 K and A$_v$=5-50 mag.}
     \label{fig:p1_global_cr}
 \end{figure*}
%%%%%%%%%%%%%%%%%%%%%%%%%%%%%%%%%%%%%%%%%%%%%
\begin{figure*}[!ht]
   \centering
     %\addtolength{\leftskip} {-8cm}
    %\addtolength{\rightskip}{-8.5cm}
     \includegraphics[width=\textwidth]{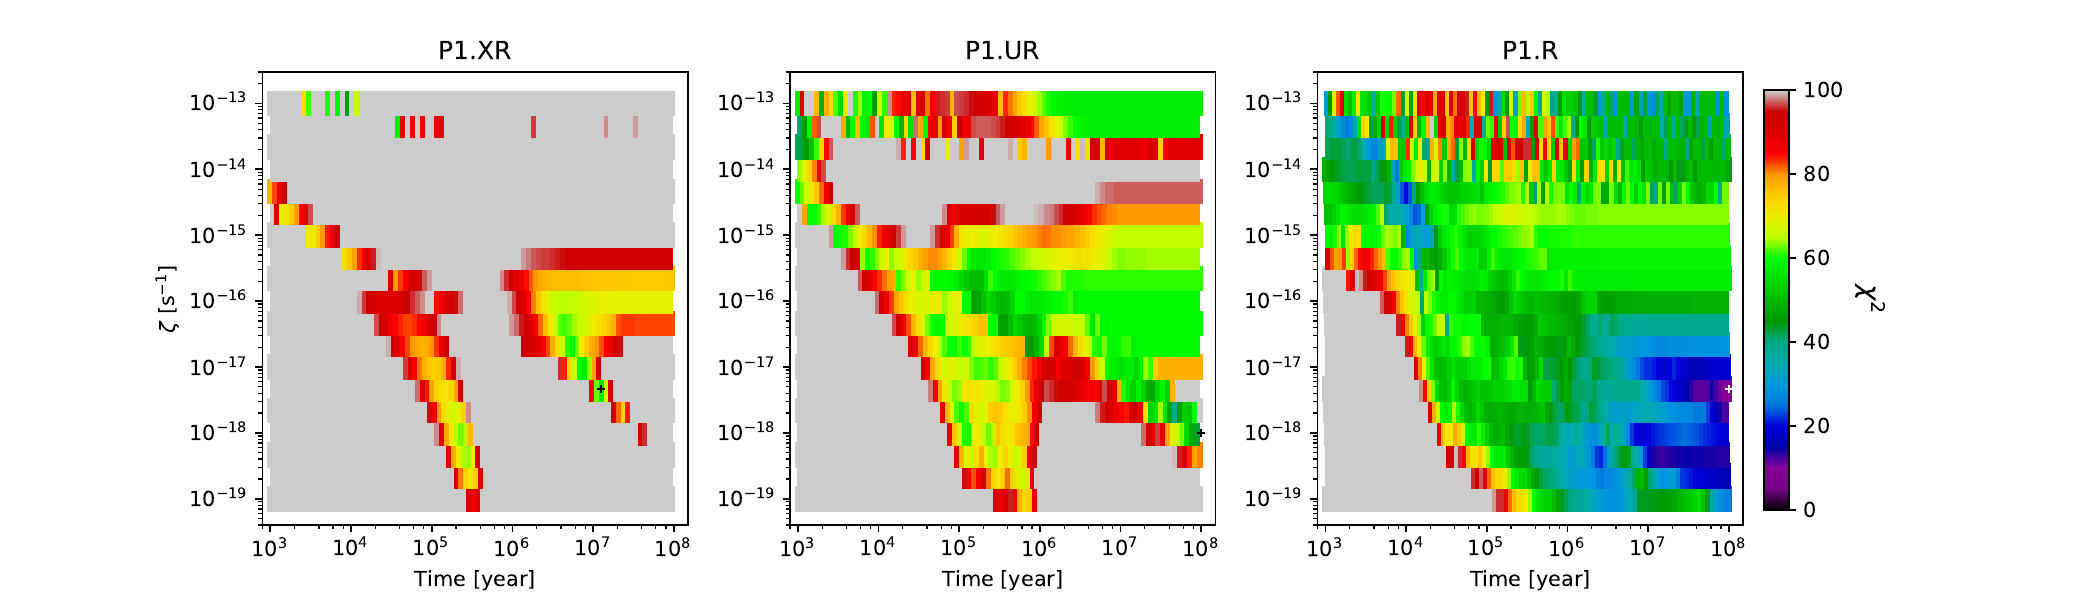}
     %\vspace{0.01cm}
     \caption{\tiny Distribution of $\zeta$ associated with $\chi^2$ using abundances of all species at P1, XR) Extra-Restricted area at which n$_H$ = 1.0e5 cm$^{-3}$, T=15 K and A$_v$=20 mag are held to be fixes and $\zeta$ has been changed, UR) Ultra-Restricted area at which n$_H$=4.6e4,1.0e5,2.2e5 cm$^{-3}$, T=10,15,20 K and A$_v$=10,20,50 mag, R) Restricted area at which n$_H$=1.0e4e4-1.0e6 cm$^{-3}$, T=10-50 K and A$_v$=5-50 mag.}
     \label{fig:p1_global_cr_all}
 \end{figure*}
 %%%%%%%%%%%%%%%%%%%%%%%%%%%%%%%%%%%%%%%%%%%%%%%%%%%%
 %%%%%%%%%%%%%%%%%%%%%%%%%%%%%%%%%%%%%%%%%%%%%%%%%%%%%

%%%%%%%%%%%%%%%%%%%%%%%%%%%%%%%%%%%%%%%%%%%%%

%%%%%%%%%%%%%%%%%%%%%%%%%%%%%%%%%%%%%%%%%%%%%
%%%%%%%%%%%%%%%%%%%%%%%%%%%%%%%%%%%%%%%%%%%%%

\begin{figure*}[!ht]
   \centering
     %\addtolength{\leftskip} {-8cm}
    %\addtolength{\rightskip}{-8.5cm}
     \includegraphics[width=\textwidth]{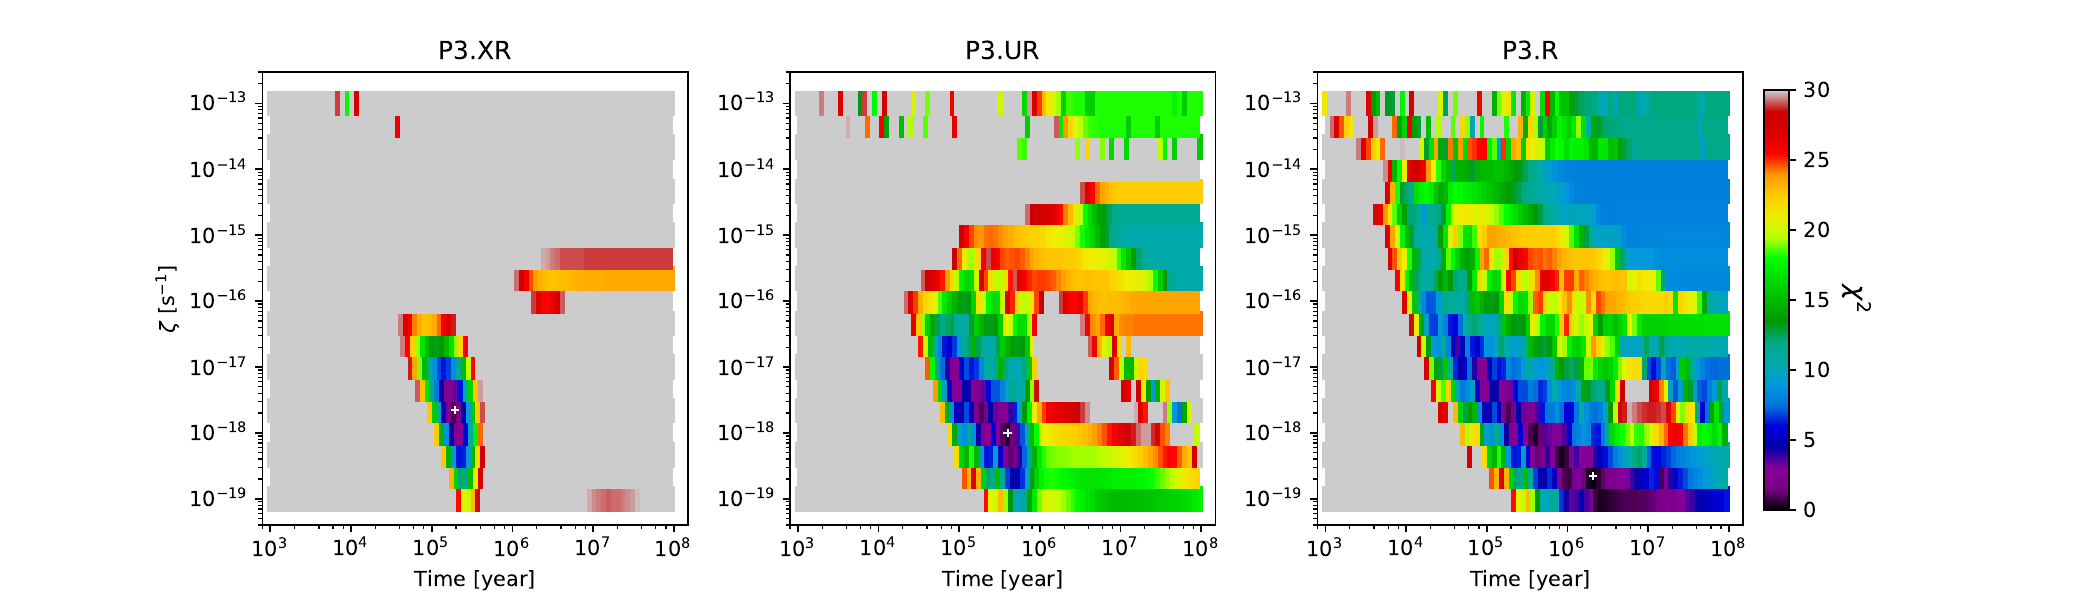}
     %\vspace{0.01cm}
     \caption{\tiny Distribution of $\zeta$ associated with $\chi^2$ using abundances of three main species CO, HCO$^+$ and N$_2$H$^+$ at P3, XR) Extra-Restricted area at which n$_H$ = 1.0e5 cm$^{-3}$, T=15 K and A$_v$=20 mag are held to be fixes and $\zeta$ has been changed, UR) Ultra-Restricted area at which n$_H$=4.6e4,1.0e5,2.2e5 cm$^{-3}$, T=10,15,20 K and A$_v$=10,20,50 mag, R) Restricted area at which n$_H$=1.0e4e4-1.0e6 cm$^{-3}$, T=10-50 K and A$_v$=5-50 mag.}
     \label{fig:p3_global_cr}
 \end{figure*}
%%%%%%%%%%%%%%%%%%%%%%%%%%%%%%%%%%%%%%%%%%%%%
%%%%%%%%%%%%%%%%%%%%%%%%%%%%%%%%%%%%%%%%%%%%%
\begin{figure*}[!ht]
   \centering
     %\addtolength{\leftskip} {-8cm}
    %\addtolength{\rightskip}{-8.5cm}
     \includegraphics[width=\textwidth]{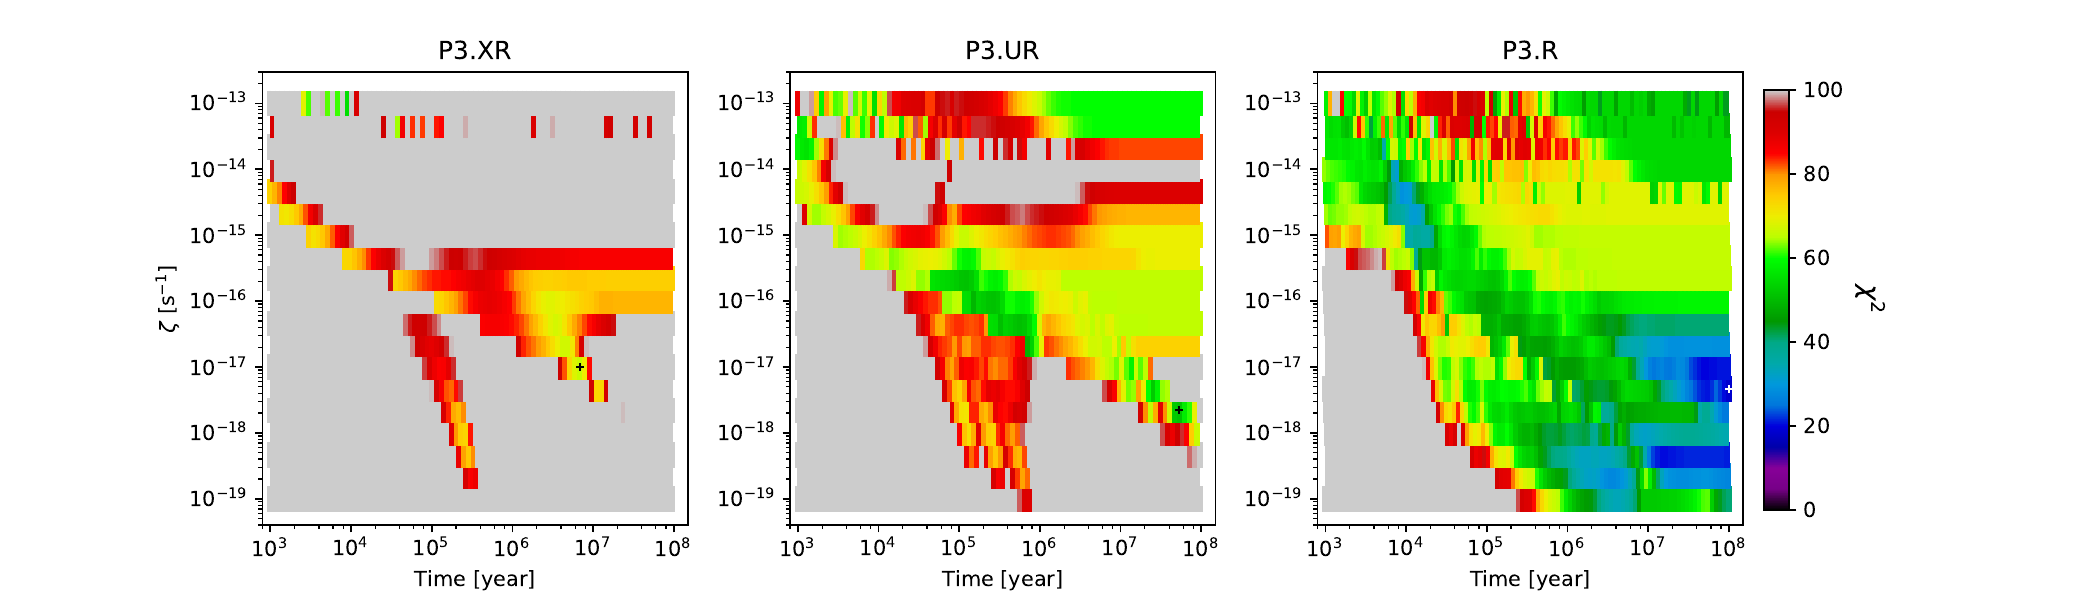}
     %\vspace{0.01cm}
     \caption{\tiny Distribution of $\zeta$ associated with $\chi^2$ using abundances of all species at P3, XR) Extra-Restricted area at which n$_H$ = 1.0e5 cm$^{-3}$, T=15 K and A$_v$=20 mag are held to be fixes and $\zeta$ has been changed, UR) Ultra-Restricted area at which n$_H$=4.6e4,1.0e5,2.2e5 cm$^{-3}$, T=10,15,20 K and A$_v$=10,20,50 mag, R) Restricted area at which n$_H$=1.0e4e4-1.0e6 cm$^{-3}$, T=10-50 K and A$_v$=5-50 mag.}
     \label{fig:p3_global_cr_all}
 \end{figure*}
%%%%%%%%%%%%%%%%%%%%%%%%%%%%%%%%%%%%%%%%%%%%%%%%%%%%%%%%%%
%%%%%%%%%%%%%%%%%%%%%%%%%%%%%%%%%%%%%%%%%%%%%%%%%%%%%%%%%%%
\begin{figure*}[!ht]
   \centering
     %\addtolength{\leftskip} {-8cm}
    %\addtolength{\rightskip}{-8.5cm}
     \includegraphics[width=\textwidth]{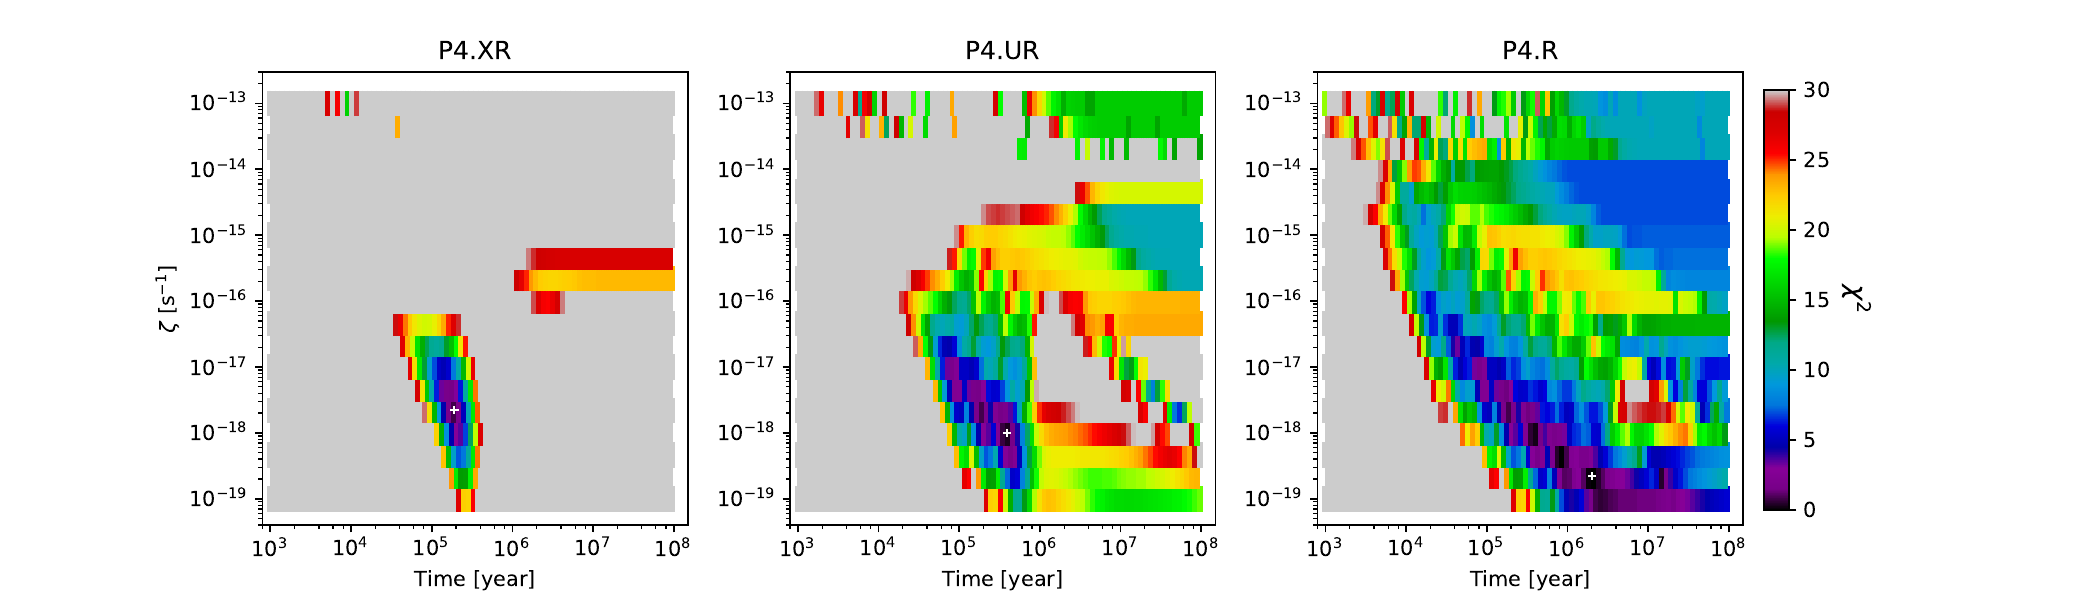}
     %\vspace{0.01cm}
     \caption{\tiny Distribution of $\zeta$ associated with $\chi^2$ using abundances of three main species CO, HCO$^+$ and N$_2$H$^+$ at P4, XR) Extra-Restricted area at which n$_H$ = 1.0e5 cm$^{-3}$, T=15 K and A$_v$=20 mag are held to be fixes and $\zeta$ has been changed, UR) Ultra-Restricted area at which n$_H$=4.6e4,1.0e5,2.2e5 cm$^{-3}$, T=10,15,20 K and A$_v$=10,20,50 mag, R) Restricted area at which n$_H$=1.0e4e4-1.0e6 cm$^{-3}$, T=10-50 K and A$_v$=5-50 mag.}
     \label{fig:p4_global_cr}
 \end{figure*}
%%%%%%%%%%%%%%%%%%%%%%%%%%%%%%%%%%%%%%%%%%%%%
%%%%%%%%%%%%%%%%%%%%%%%%%%%%%%%%%%%%%%%%%%%%%
\begin{figure*}[!ht]
   \centering
     %\addtolength{\leftskip} {-8cm}
    %\addtolength{\rightskip}{-8.5cm}
     \includegraphics[width=\textwidth]{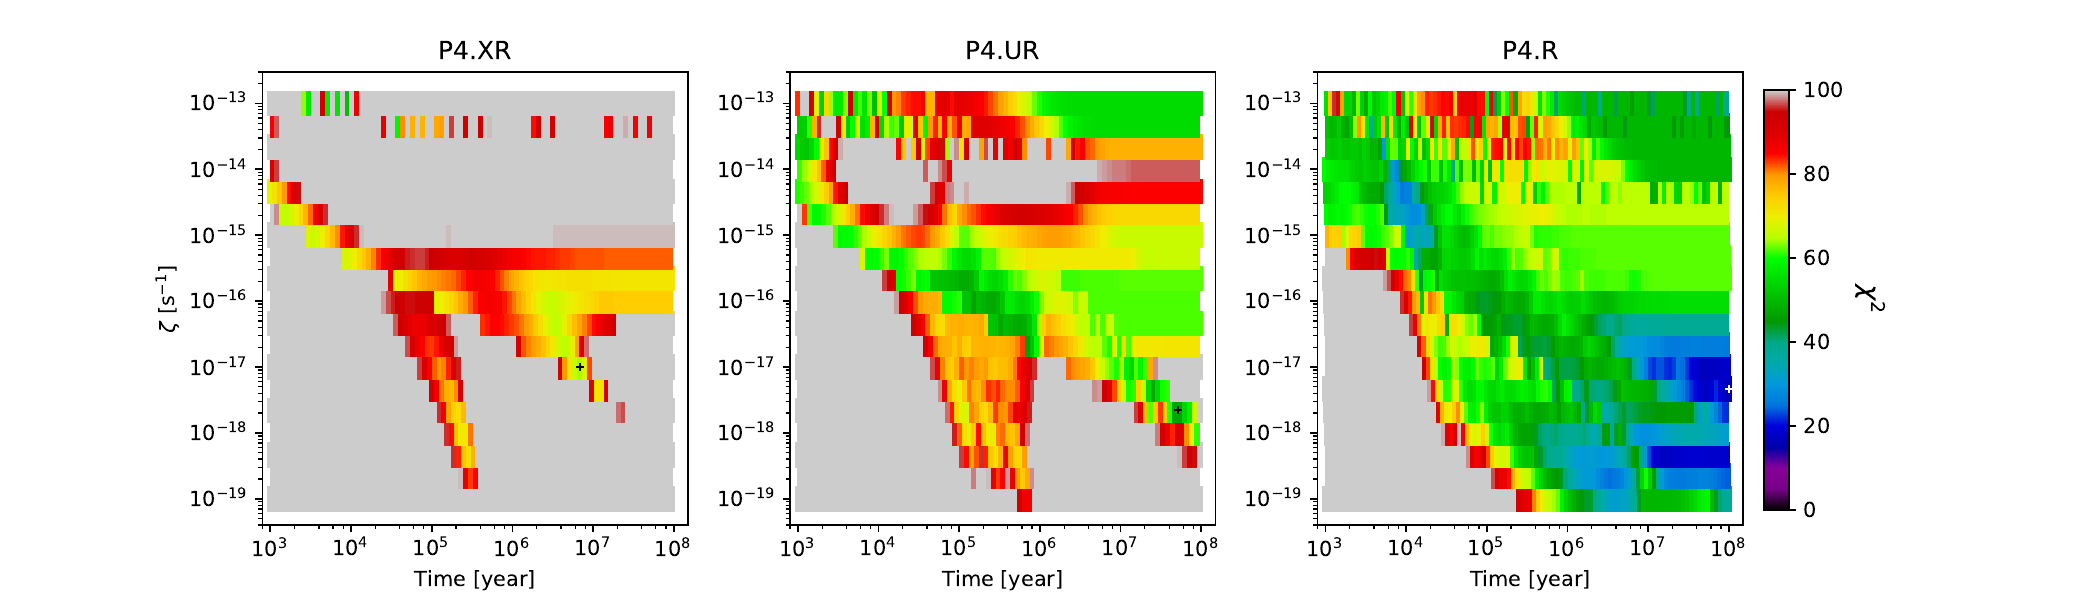}
     %\vspace{0.01cm}
     \caption{\tiny Distribution of $\zeta$ associated with $\chi^2$ using abundances of all species at P4, XR) Extra-Restricted area at which n$_H$ = 1.0e5 cm$^{-3}$, T=15 K and A$_v$=20 mag are held to be fixes and $\zeta$ has been changed, UR) Ultra-Restricted area at which n$_H$=4.6e4,1.0e5,2.2e5 cm$^{-3}$, T=10,15,20 K and A$_v$=10,20,50 mag, R) Restricted area at which n$_H$=1.0e4e4-1.0e6 cm$^{-3}$, T=10-50 K and A$_v$=5-50 mag.}
     \label{fig:p4_global_cr_all}
 \end{figure*}
%%%%%%%%%%%%%%%%%%%%%%%%%%%%%%%%%%%%%%%%%%%%%%%%%%%%
%%%%%%%%%%%%%%%%%%%%%%%%%%%%%%%%%%%%%%%%%%%%%%%%%%%%%
\begin{figure*}[!ht]
   \centering
     %\addtolength{\leftskip} {-8cm}
    %\addtolength{\rightskip}{-8.5cm}
     \includegraphics[width=\textwidth]{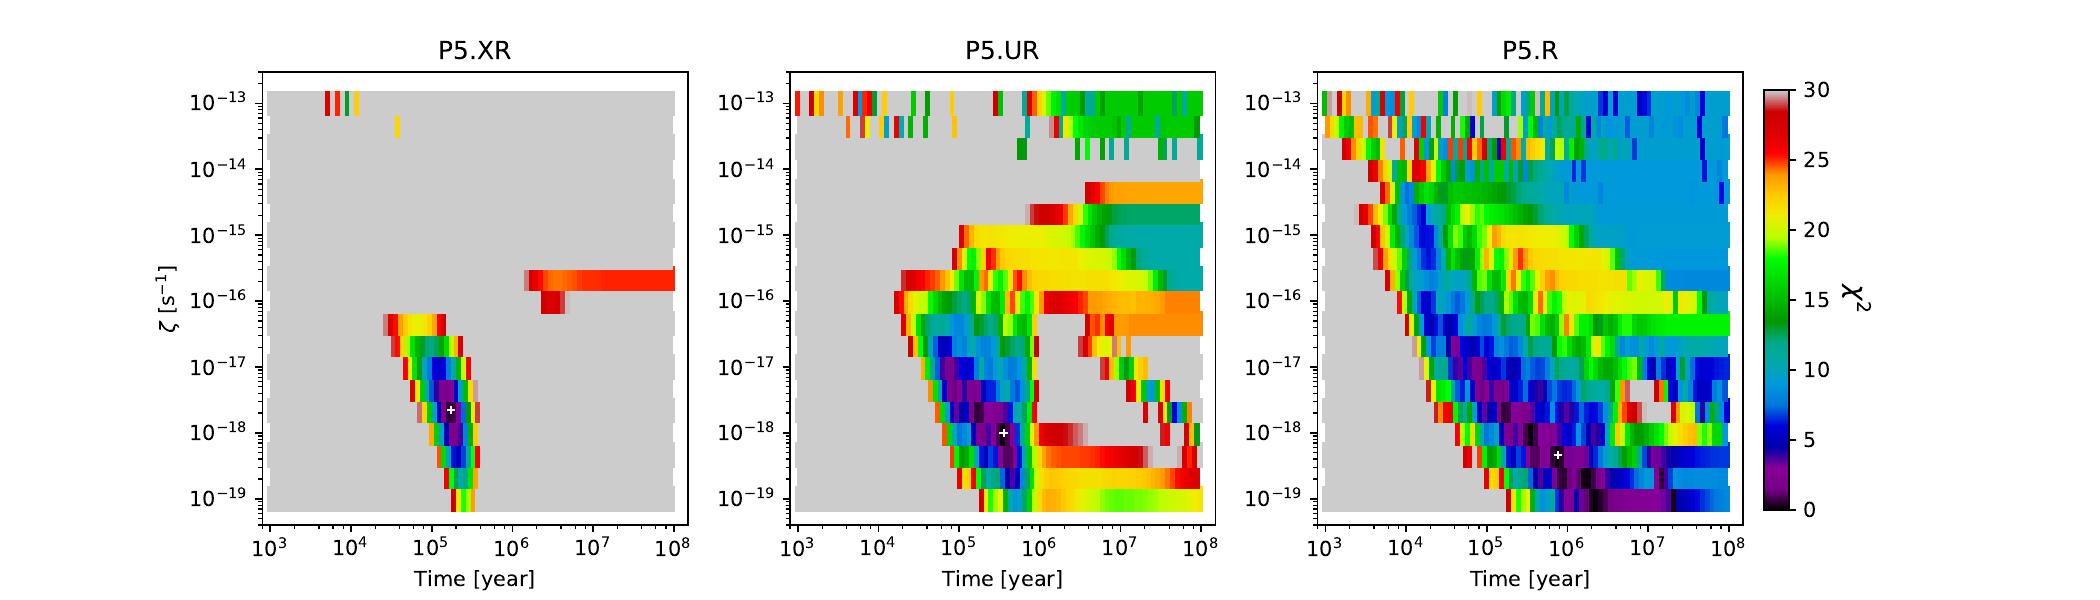}
     %\vspace{0.01cm}
     \caption{\tiny Distribution of $\zeta$ associated with $\chi^2$ using abundances of three main species CO, HCO$^+$ and N$_2$H$^+$ at P5, XR) Extra-Restricted area at which n$_H$ = 1.0e5 cm$^{-3}$, T=15 K and A$_v$=20 mag are held to be fixes and $\zeta$ has been changed, UR) Ultra-Restricted area at which n$_H$=4.6e4,1.0e5,2.2e5 cm$^{-3}$, T=10,15,20 K and A$_v$=10,20,50 mag, R) Restricted area at which n$_H$=1.0e4e4-1.0e6 cm$^{-3}$, T=10-50 K and A$_v$=5-50 mag.}
     \label{fig:p5_global_cr}
 \end{figure*}
%%%%%%%%%%%%%%%%%%%%%%%%%%%%%%%%%%%%%%%%%%%%%
%%%%%%%%%%%%%%%%%%%%%%%%%%%%%%%%%%%%%%%%%%%%%
\begin{figure*}[!ht]
   \centering
     %\addtolength{\leftskip} {-8cm}
    %\addtolength{\rightskip}{-8.5cm}
     \includegraphics[width=\textwidth]{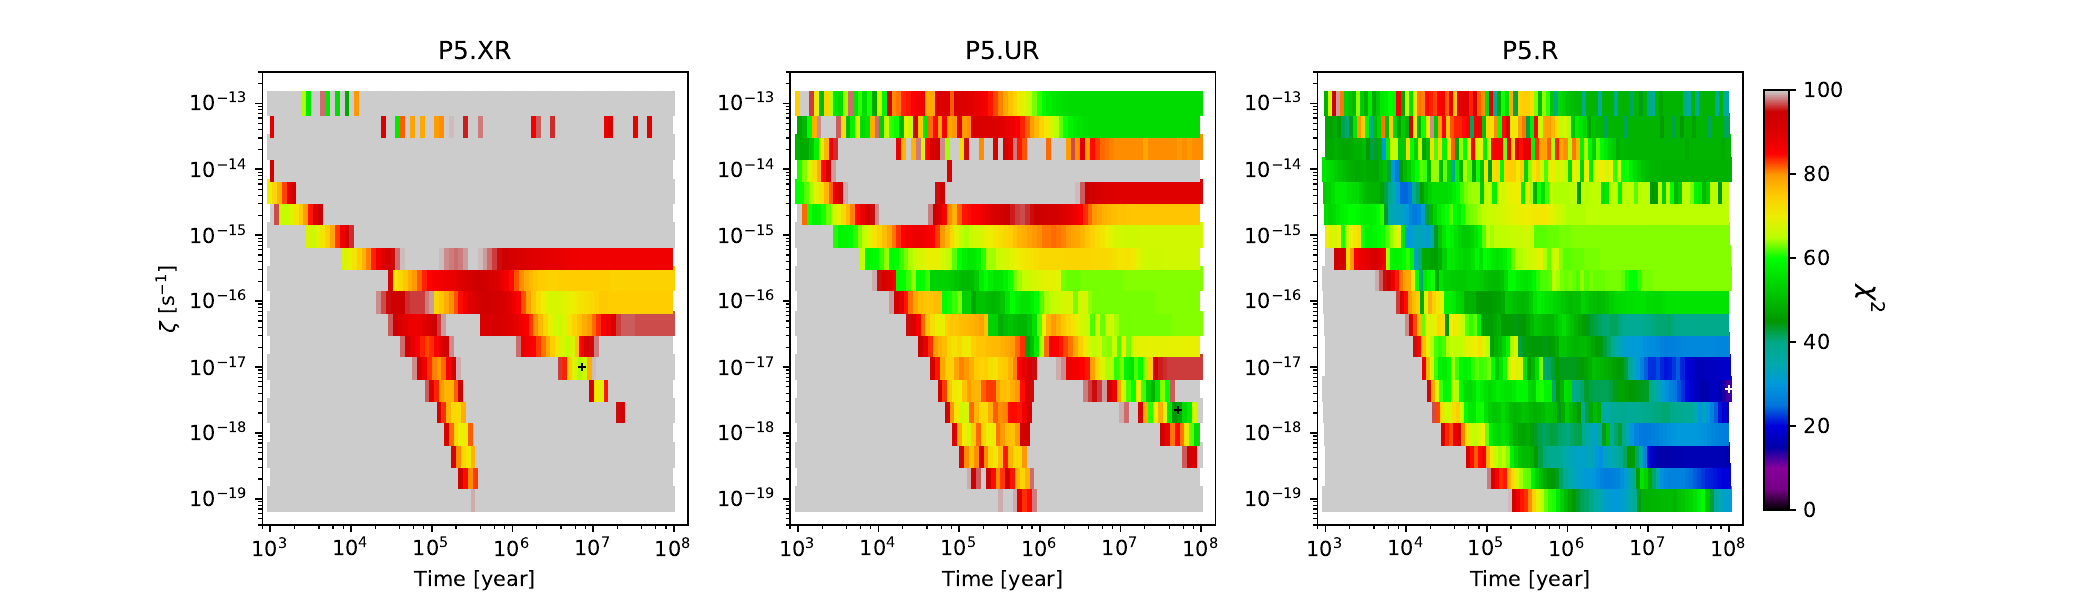}
     %\vspace{0.01cm}
     \caption{\tiny Distribution of $\zeta$ associated with $\chi^2$ using abundances of all species at P5, XR) Extra-Restricted area at which n$_H$ = 1.0e5 cm$^{-3}$, T=15 K and A$_v$=20 mag are held to be fixes and $\zeta$ has been changed, UR) Ultra-Restricted area at which n$_H$=4.6e4,1.0e5,2.2e5 cm$^{-3}$, T=10,15,20 K and A$_v$=10,20,50 mag, R) Restricted area at which n$_H$=1.0e4e4-1.0e6 cm$^{-3}$, T=10-50 K and A$_v$=5-50 mag.}
     \label{fig:p5_global_cr_all}
 \end{figure*}
%%%%%%%%%%%%%%%%%%%%%%%%%%%%%%%%%%%%%%%%%%%%%%%%%%%%
%%%%%%%%%%%%%%%%%%%%%%%%%%%%%%%%%%%%%%%%%%%%%%%%%%%%%

%%%%%%%%%%%%%%%%%%%%%%%%%%%%%%%%%%%%%%%%%%%%%
%%
%%%%%%%%%%%%%%%%%%%%%%%%%%%%%%%%%%%%%%%%%%%%%%%%%%%%%
\begin{figure*}[!ht]
   \centering
     %\addtolength{\leftskip} {-8cm}
    %\addtolength{\rightskip}{-8.5cm}
     \includegraphics[width=\textwidth]{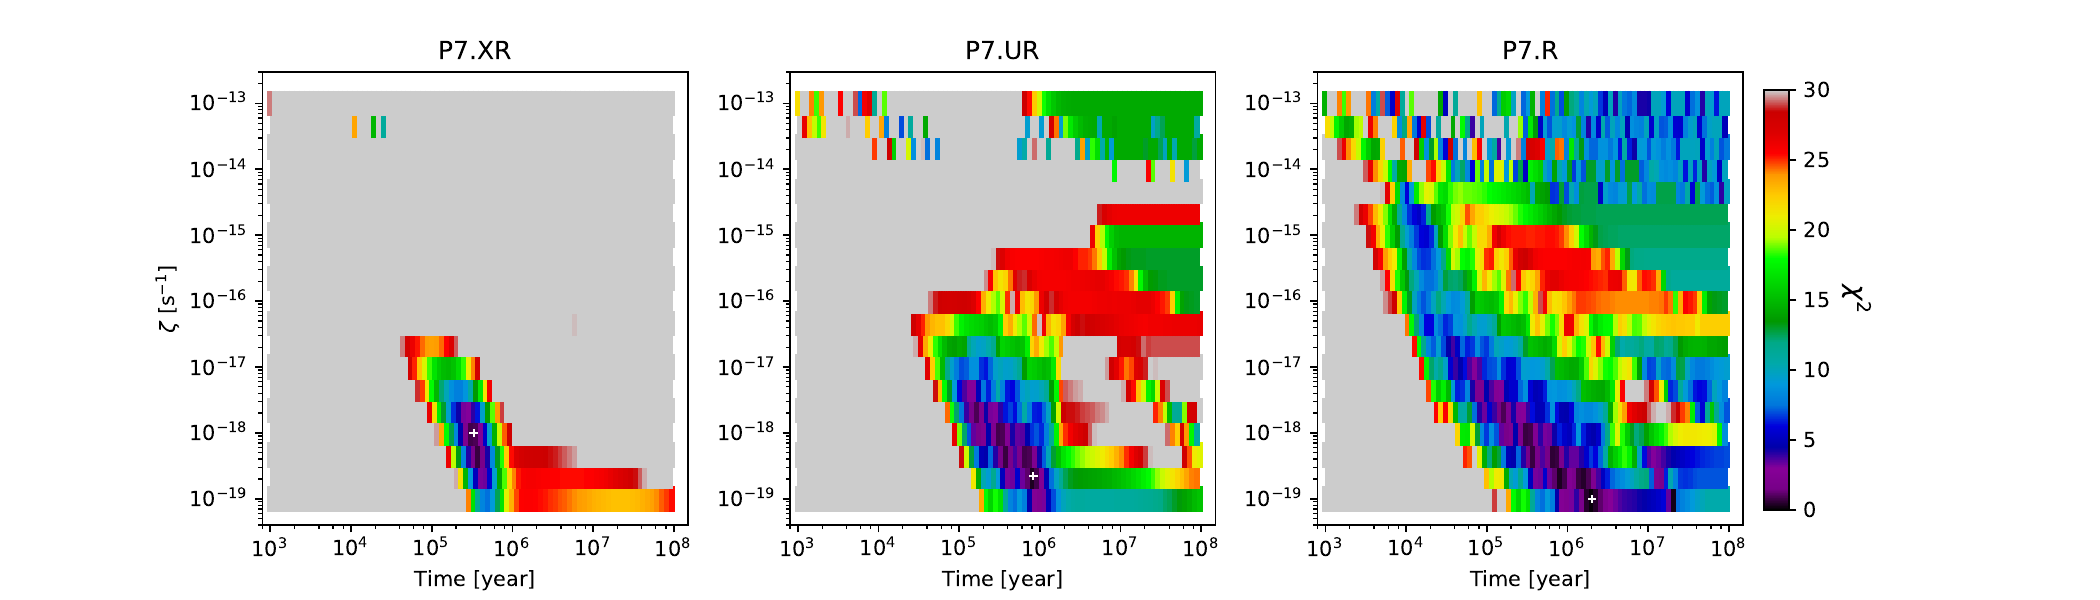}
     %\vspace{0.01cm}
     \caption{\tiny Distribution of $\zeta$ associated with $\chi^2$ using abundances of three main species CO, HCO$^+$ and N$_2$H$^+$ at P7, XR) Extra-Restricted area at which n$_H$ = 4.6e4 cm$^{-3}$, T=15 K and A$_v$=10 mag are held to be fixes and $\zeta$ has been changed, UR) Ultra-Restricted area at which n$_H$=2.2e4,4.6e4,1.0e5 cm$^{-3}$, T=10,15,20 K and A$_v$=7,10,20 mag, R) Restricted area at which n$_H$=1.0e4e4-1.0e6 cm$^{-3}$, T=10-50 K and A$_v$=5-50 mag.}
     \label{fig:p7_global_cr}
 \end{figure*}
%%%%%%%%%%%%%%%%%%%%%%%%%%%%%%%%%%%%%%%%%%%%%
%%%%%%%%%%%%%%%%%%%%%%%%%%%%%%%%%%%%%%%%%%%%%
\begin{figure*}[!ht]
   \centering
     %\addtolength{\leftskip} {-8cm}
    %\addtolength{\rightskip}{-8.5cm}
     \includegraphics[width=\textwidth]{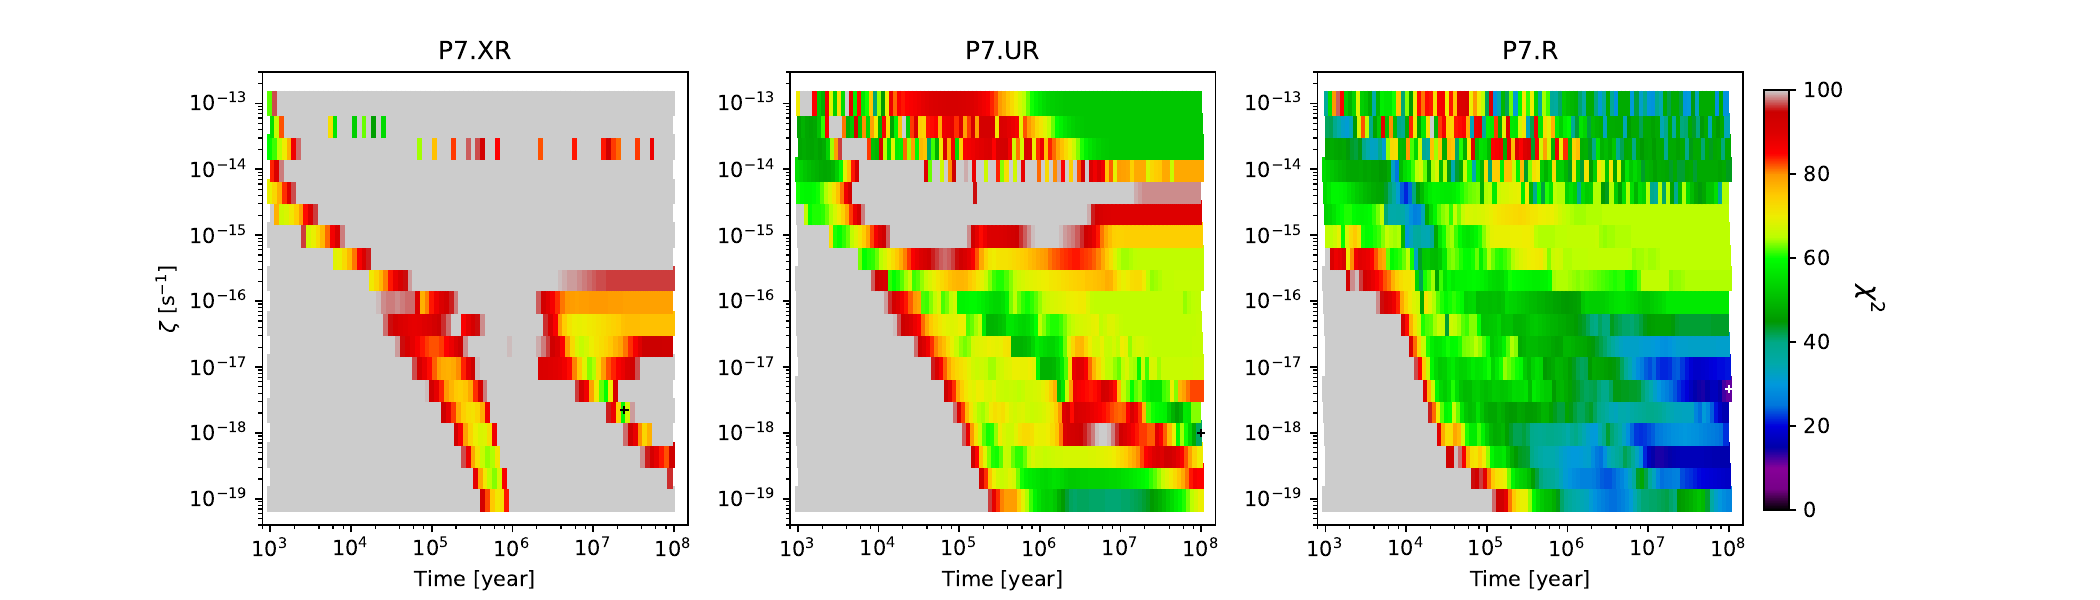}
     %\vspace{0.01cm}
     \caption{\tiny Distribution of $\zeta$ associated with $\chi^2$ using abundances of all species at P7, XR) Extra-Restricted area at which n$_H$ = 4.6e4 cm$^{-3}$, T=15 K and A$_v$=10 mag are held to be fixes and $\zeta$ has been changed, UR) Ultra-Restricted area at which n$_H$=2.2e4,4.6e4,1.0e5 cm$^{-3}$, T=10,15,20 K and A$_v$=7,10,20 mag, R) Restricted area at which n$_H$=1.0e4e4-1.0e6 cm$^{-3}$, T=10-50 K and A$_v$=5-50 mag.}
     \label{fig:p7_global_cr_all}
 \end{figure*}
%%%%%%%%%%%%%%%%%%%%%%%%%%%%%%%%%%%%%%%%%%%%%%%%%%%%
%%%%%%%%%%%%%%%%%%%%%%%%%%%%%%%%%%%%%%%%%%%%%%%%%%%%%
\begin{figure*}[!ht]
   \centering
     %\addtolength{\leftskip} {-8cm}
    %\addtolength{\rightskip}{-8.5cm}
     \includegraphics[width=\textwidth]{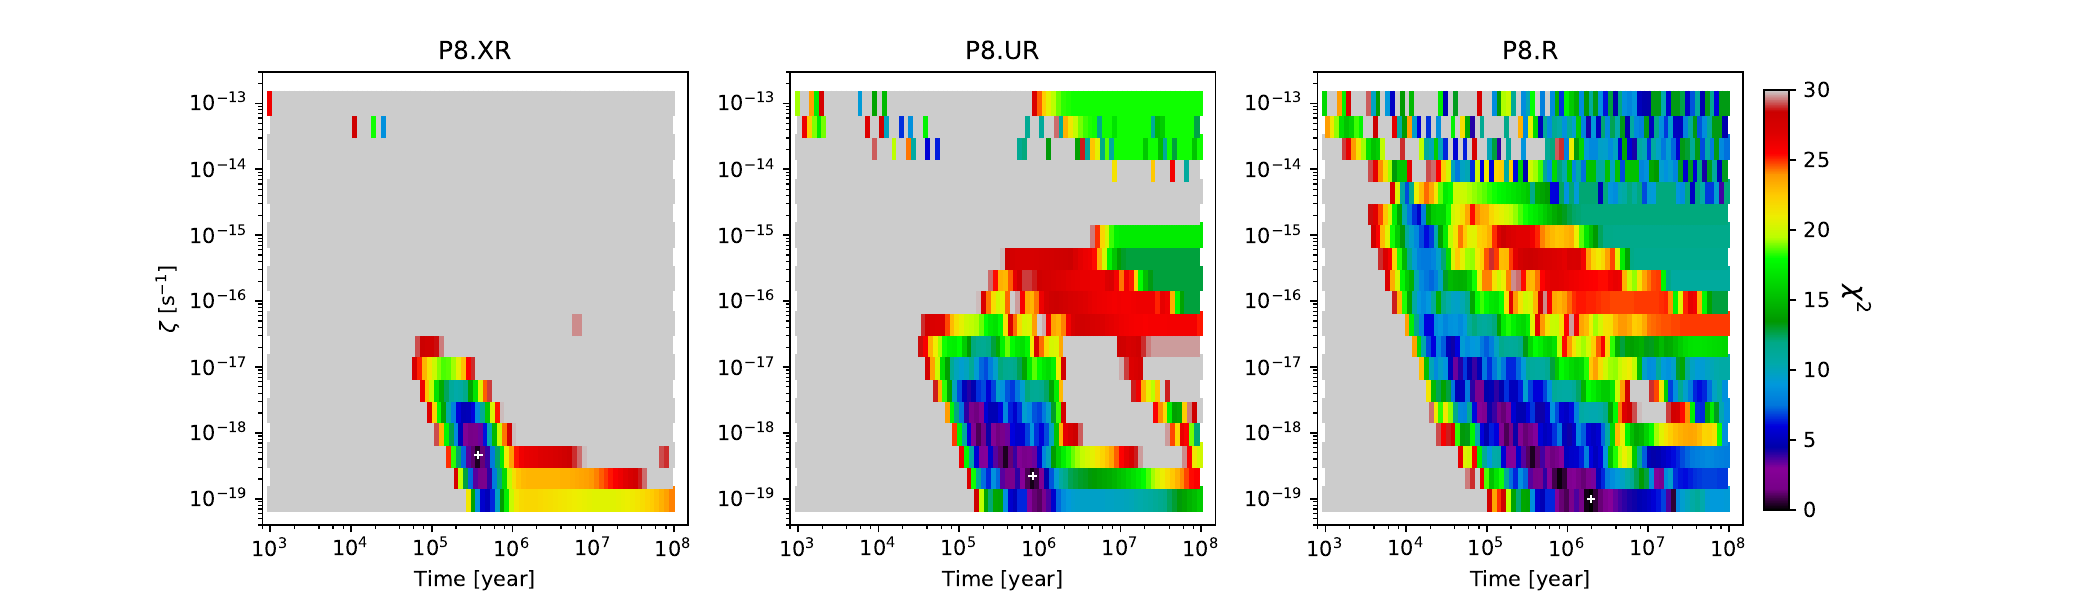}
     %\vspace{0.01cm}
     \caption{\tiny Distribution of $\zeta$ associated with $\chi^2$ using abundances of three main species CO, HCO$^+$ and N$_2$H$^+$ at P8, XR) Extra-Restricted area at which n$_H$ = 4.6e4 cm$^{-3}$, T=15 K and A$_v$=10 mag are held to be fixes and $\zeta$ has been changed, UR) Ultra-Restricted area at which n$_H$=2.2e4,4.6e4,1.0e5 cm$^{-3}$, T=10,15,20 K and A$_v$=7,10,20 mag, R) Restricted area at which n$_H$=1.0e4e4-1.0e6 cm$^{-3}$, T=10-50 K and A$_v$=5-50 mag.}
     \label{fig:p8_global_cr}
 \end{figure*}
%%%%%%%%%%%%%%%%%%%%%%%%%%%%%%%%%%%%%%%%%%%%%
%%%%%%%%%%%%%%%%%%%%%%%%%%%%%%%%%%%%%%%%%%%%%
\begin{figure*}[!ht]
   \centering
     %\addtolength{\leftskip} {-8cm}
    %\addtolength{\rightskip}{-8.5cm}
     \includegraphics[width=\textwidth]{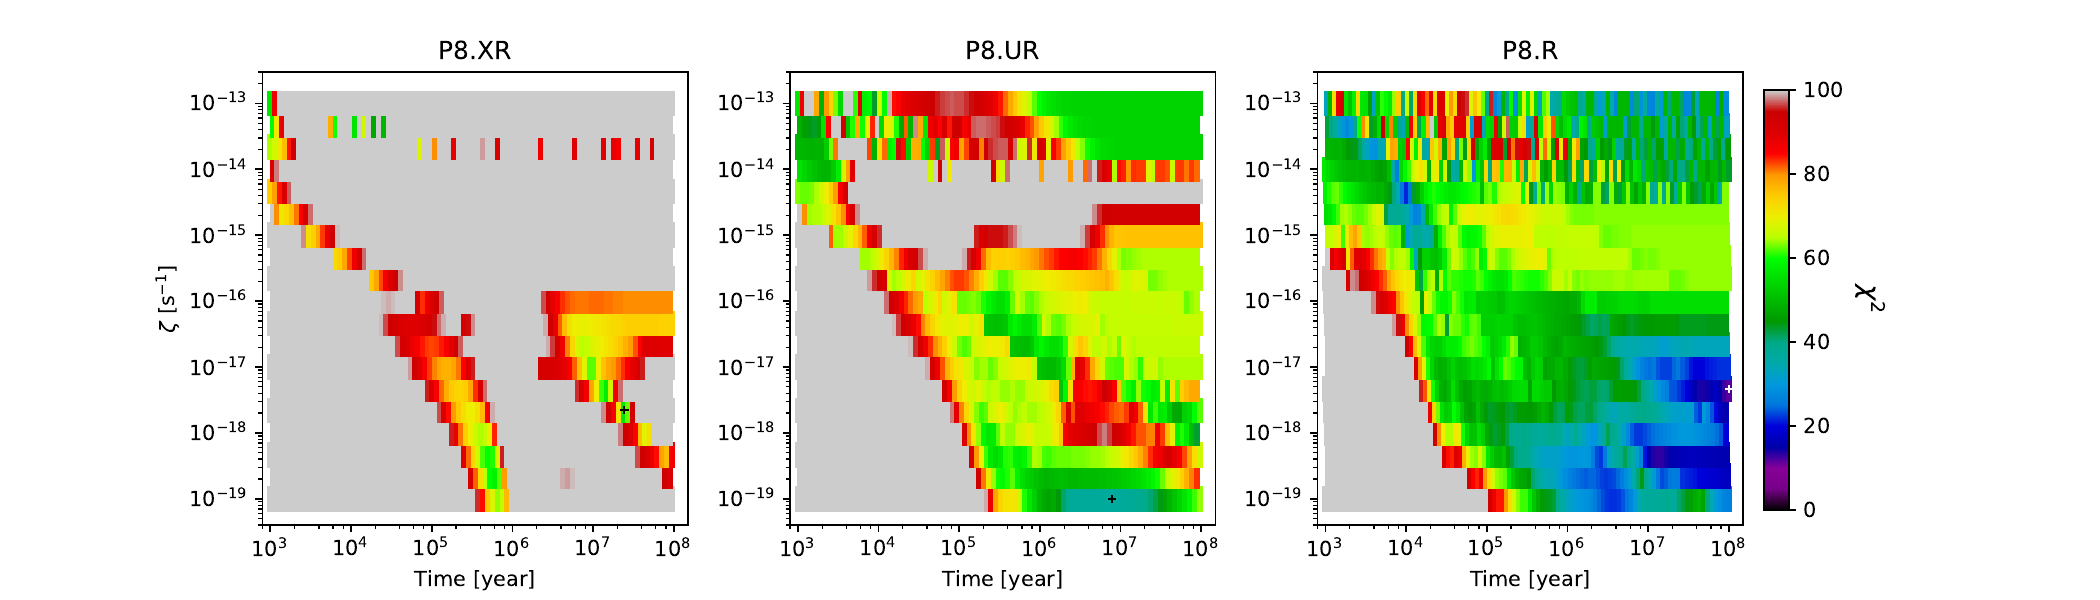}
     %\vspace{0.01cm}
     \caption{\tiny Distribution of $\zeta$ associated with $\chi^2$ using abundances of all species at P8, XR) Extra-Restricted area at which n$_H$ = 4.6e4 cm$^{-3}$, T=15 K and A$_v$=10 mag are held to be fixes and $\zeta$ has been changed, UR) Ultra-Restricted area at which n$_H$=2.2e4,4.6e4,1.0e5 cm$^{-3}$, T=10,15,20 K and A$_v$=7,10,20 mag, R) Restricted area at which n$_H$=1.0e4e4-1.0e6 cm$^{-3}$, T=10-50 K and A$_v$=5-50 mag.}
     \label{fig:p8_global_cr_all}
 \end{figure*}
%%%%%%%%%%%%%%%%%%%%%%%%%%%%%%%%%%%%%%%%%%%%%%%%%%%%
%%%%%%%%%%%%%%%%%%%%%%%%%%%%%%%%%%%%%%%%%%%%%%%%%%%%%
\begin{figure*}[!ht]
   \centering
     %\addtolength{\leftskip} {-8cm}
    %\addtolength{\rightskip}{-8.5cm}
     \includegraphics[width=\textwidth]{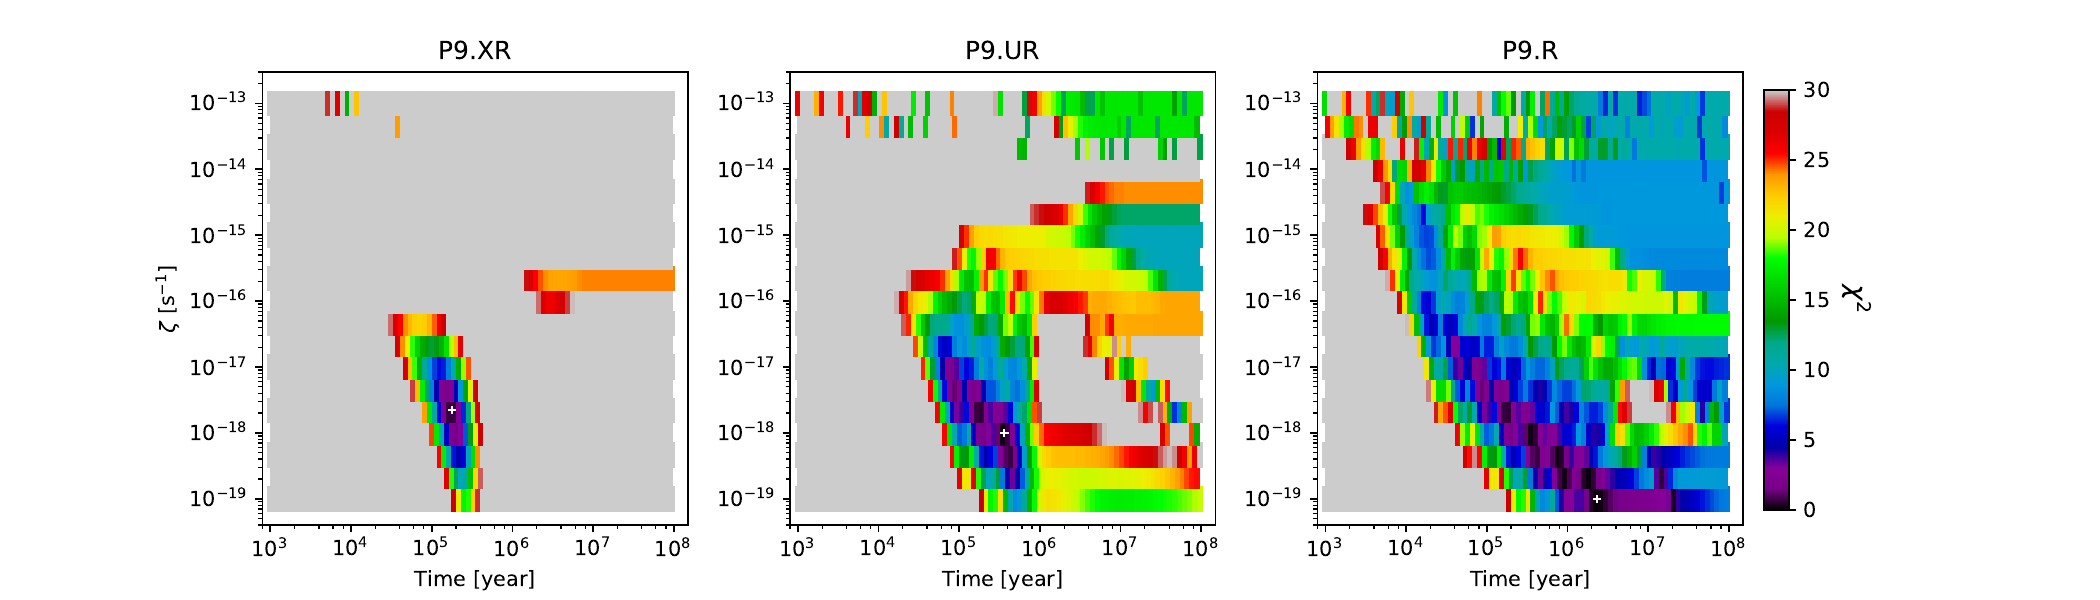}
     %\vspace{0.01cm}
     \caption{\tiny Distribution of $\zeta$ associated with $\chi^2$ using abundances of three main species CO, HCO$^+$ and N$_2$H$^+$ at P9, XR) Extra-Restricted area at which n$_H$ = 1.0e5 cm$^{-3}$, T=15 K and A$_v$=20 mag are held to be fixes and $\zeta$ has been changed, UR) Ultra-Restricted area at which n$_H$=4.6e4,1.0e5,2.2e5 cm$^{-3}$, T=10,15,20 K and A$_v$=10,20,50 mag, R) Restricted area at which n$_H$=1.0e4e4-1.0e6 cm$^{-3}$, T=10-50 K and A$_v$=5-50 mag.}
     \label{fig:p9_global_cr}
 \end{figure*}
%%%%%%%%%%%%%%%%%%%%%%%%%%%%%%%%%%%%%%%%%%%%%
%%%%%%%%%%%%%%%%%%%%%%%%%%%%%%%%%%%%%%%%%%%%%
\begin{figure*}[!ht]
   \centering
     %\addtolength{\leftskip} {-8cm}
    %\addtolength{\rightskip}{-8.5cm}
     \includegraphics[width=\textwidth]{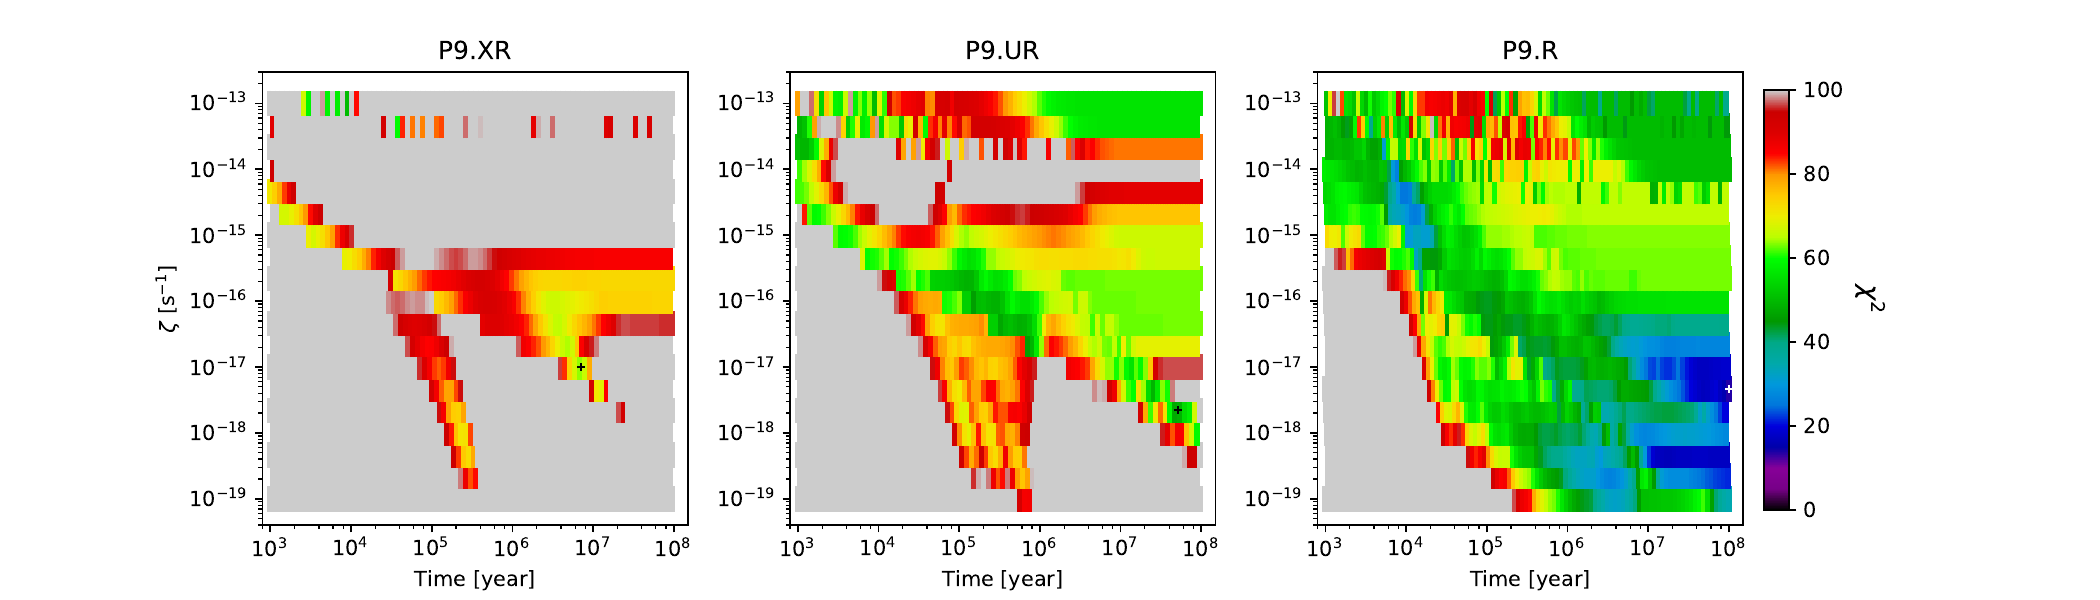}
     %\vspace{0.01cm}
     \caption{\tiny Distribution of $\zeta$ associated with $\chi^2$ using abundances of all species at P9, XR) Extra-Restricted area at which n$_H$ = 1.0e5 cm$^{-3}$, T=15 K and A$_v$=20 mag are held to be fixes and $\zeta$ has been changed, UR) Ultra-Restricted area at which n$_H$=4.6e4,1.0e5,2.2e5 cm$^{-3}$, T=10,15,20 K and A$_v$=10,20,50 mag, R) Restricted area at which n$_H$=1.0e4e4-1.0e6 cm$^{-3}$, T=10-50 K and A$_v$=5-50 mag.}
     \label{fig:p9_global_cr_all}
 \end{figure*}
%%%%%%%%%%%%%%%%%%%%%%%%%%%%%%%%%%%%%%%%%%%%%%%%%%%%
%%%%%%%%%%%%%%%%%%%%%%%%%%%%%%%%%%%%%%%%%%%%%%%%%%%%%
\begin{figure*}[!ht]
   \centering
     %\addtolength{\leftskip} {-8cm}
    %\addtolength{\rightskip}{-8.5cm}
     \includegraphics[width=\textwidth]{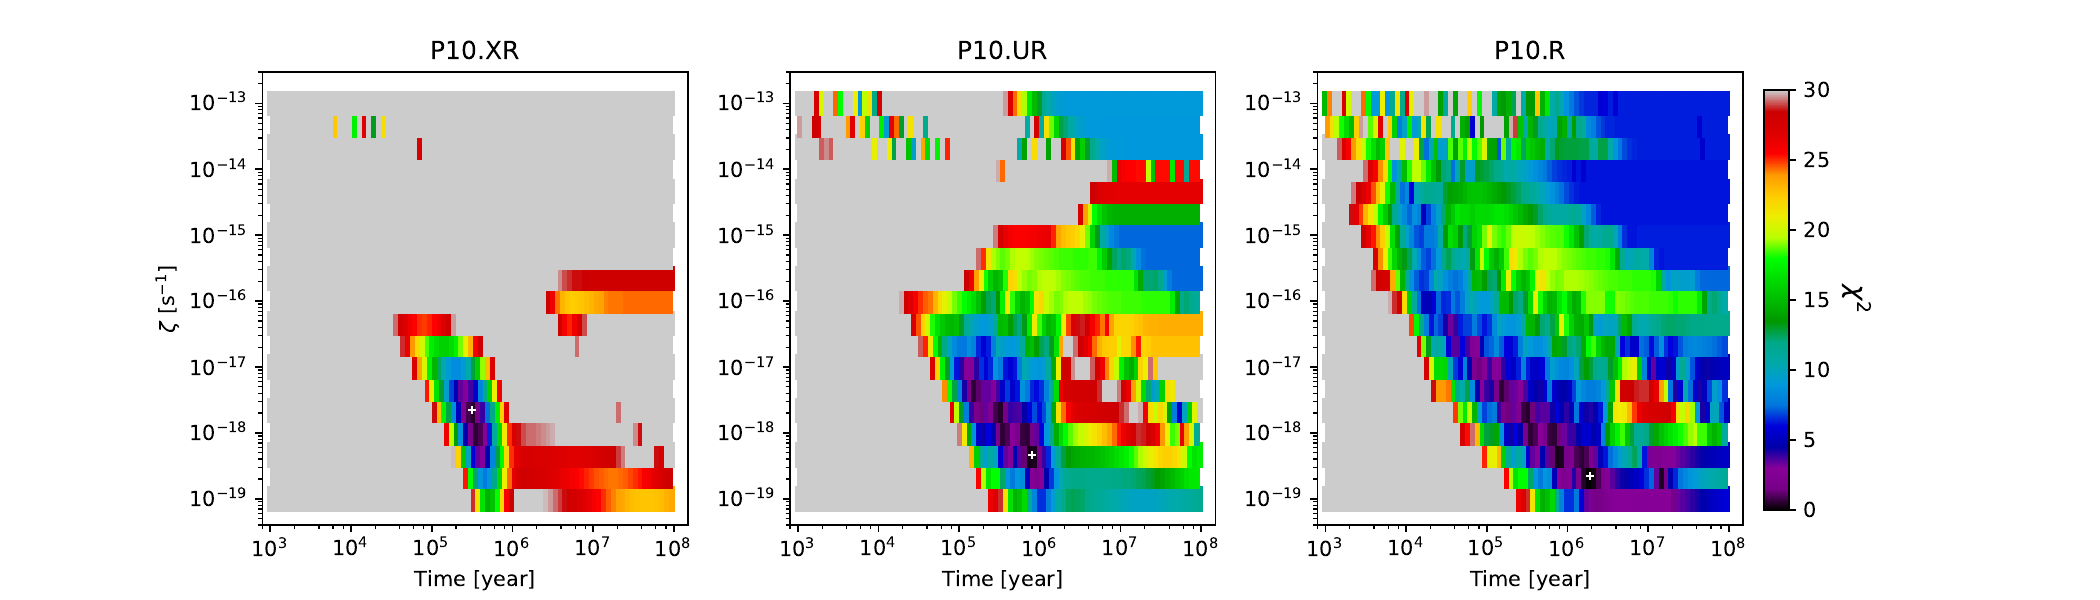}
     %\vspace{0.01cm}
     \caption{\tiny Distribution of $\zeta$ associated with $\chi^2$ using abundances of three main species CO, HCO$^+$ and N$_2$H$^+$ at P10, XR) Extra-Restricted area at which n$_H$ = 4.6e4 cm$^{-3}$, T=15 K and A$_v$=10 mag are held to be fixes and $\zeta$ has been changed, UR) Ultra-Restricted area at which n$_H$=2.2e4,4.6e4,1.0e5 cm$^{-3}$, T=10,15,20 K and A$_v$=7,10,20 mag, R) Restricted area at which n$_H$=1.0e4e4-1.0e6 cm$^{-3}$, T=10-50 K and A$_v$=5-50 mag.}
     \label{fig:p10_global_cr}
 \end{figure*}
%%%%%%%%%%%%%%%%%%%%%%%%%%%%%%%%%%%%%%%%%%%%%
%%%%%%%%%%%%%%%%%%%%%%%%%%%%%%%%%%%%%%%%%%%%%
\begin{figure*}[!ht]
   \centering
     %\addtolength{\leftskip} {-8cm}
    %\addtolength{\rightskip}{-8.5cm}
     \includegraphics[width=\textwidth]{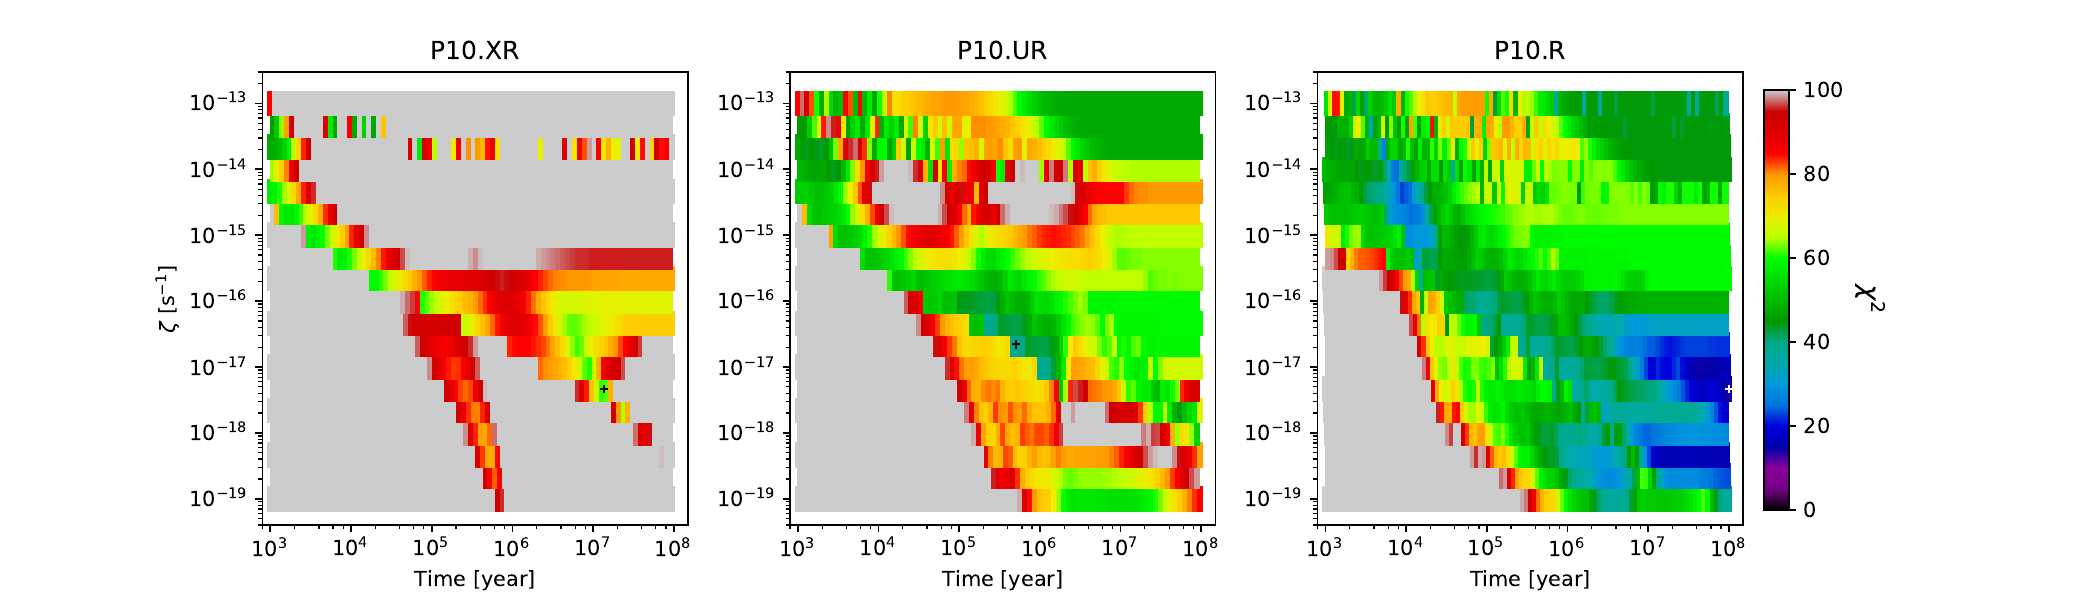}
     %\vspace{0.01cm}
     \caption{\tiny Distribution of $\zeta$ associated with $\chi^2$ using abundances of all species at P10, XR) Extra-Restricted area at which n$_H$ = 4.6e4 cm$^{-3}$, T=15 K and A$_v$=10 mag are held to be fixes and $\zeta$ has been changed, UR) Ultra-Restricted area at which n$_H$=2.2e4,4.6e4,1.0e5 cm$^{-3}$, T=10,15,20 K and A$_v$=7,10,20 mag, R) Restricted area at which n$_H$=1.0e4e4-1.0e6 cm$^{-3}$, T=10-50 K and A$_v$=5-50 mag.}
     \label{fig:p10_global_cr_all}
 \end{figure*}
%%%%%%%%%%%%%%%%%%%%%%%%%%%%%%%%%%%%%%%%%%%%%%
%%%%%%%%%%%%%%%%%%%%%%%%%%%%%%%%%%%%%%%%%%%%%%
\end{appendices}
