# Supplementary material for: Astrochemical modelling of infrared dark clouds
Source: arXiv:2111.05379 source file (2022-03-23)
Supplement: Supplementary file 3 [file appendix5.tex]

\begin{appendices}
%%%%%%%%%%%%%%%%%%%%%%%%%%%%%%%%%%%%%%%%%%%%%%%%%%%%%%%
\begin{figure*}[!ht]
   \centering
     %\addtolength{\leftskip} {-8cm}
    %\addtolength{\rightskip}{-8.5cm}
     \includegraphics[width=\textwidth]{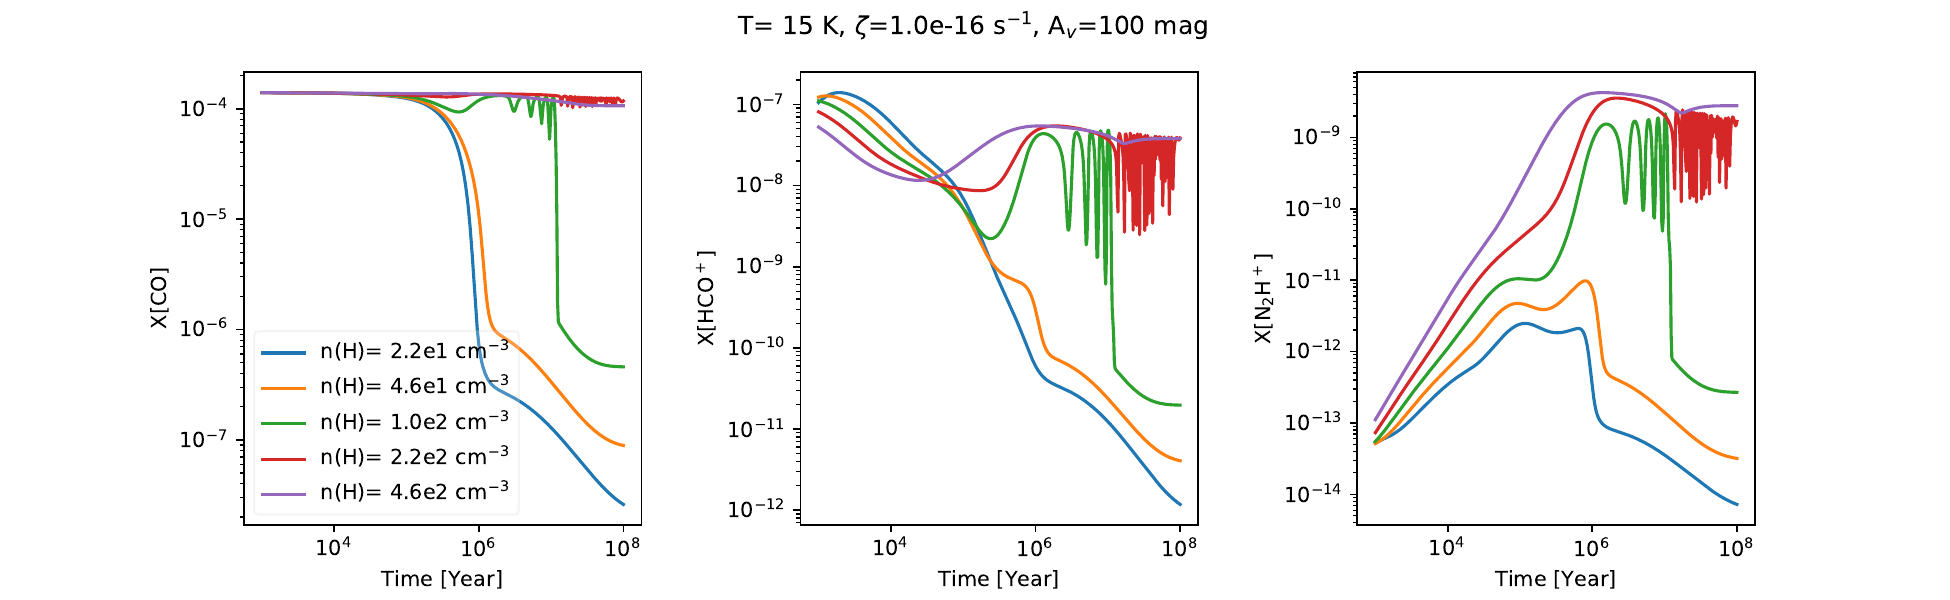}
     %\vspace{0.01cm}
     \caption{\tiny Influence of the density on the appearance of the vacillatory evolution of the species}
     \label{fig:os_n}
 \end{figure*}
%%%%%%%%%%%%%%%%%%%%%%%%%%%%%%%%%%%%%%%%%%%%%%%%%%%%%%
\begin{figure*}[!ht]
   \centering
     %\addtolength{\leftskip} {-8cm}
    %\addtolength{\rightskip}{-8.5cm}
     \includegraphics[width=\textwidth]{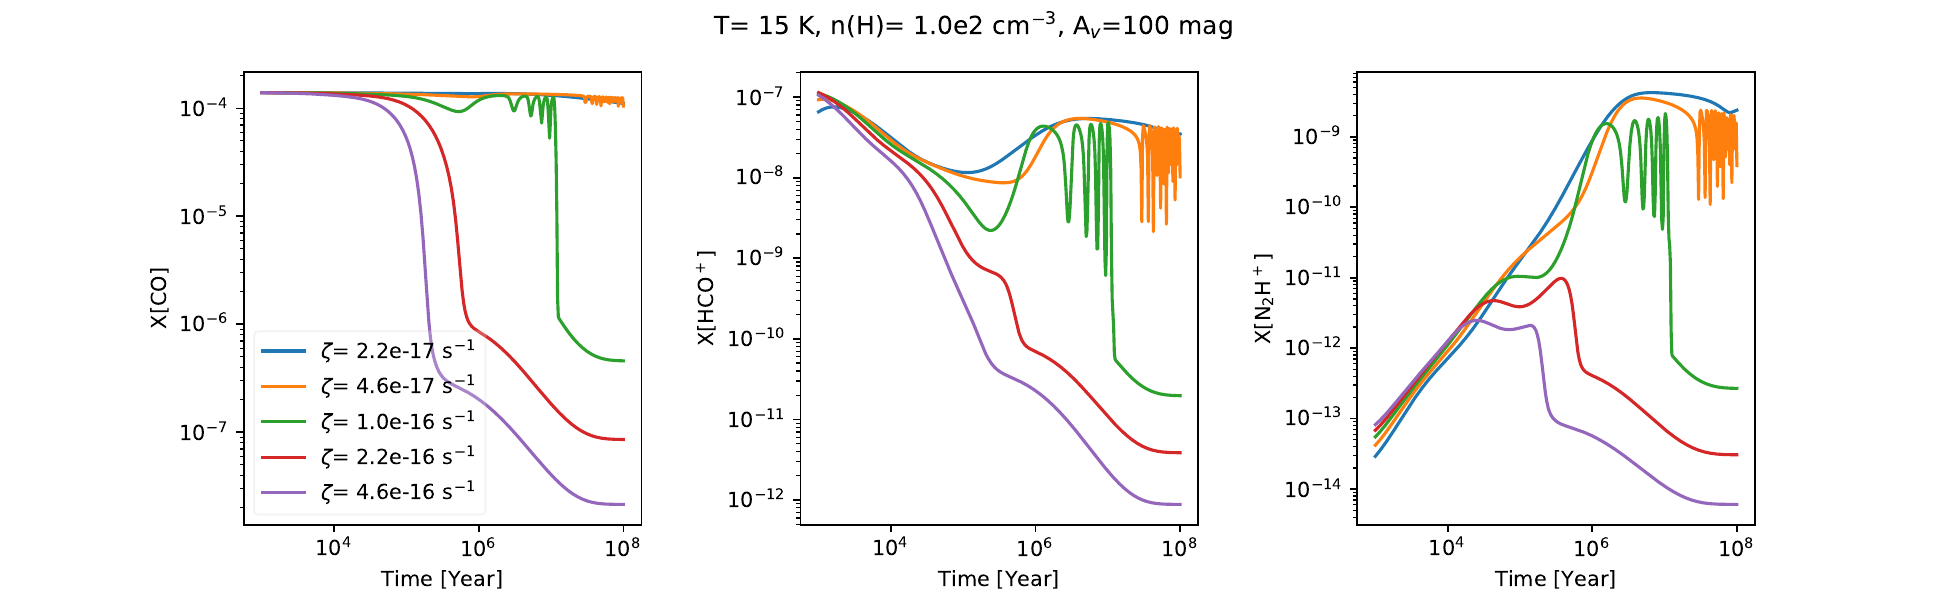}
     %\vspace{0.01cm}
     \caption{\tiny Influence of the CRIR on the appearance of the vacillatory evolution of the species}
     \label{fig:os_cr}
 \end{figure*}
%%%%%%%%%%%%%%%%%%%%%%%%%%%%%%%%%%%%%%%%%%%%%%%%
\begin{figure*}[!ht]
   \centering
     %\addtolength{\leftskip} {-8cm}
    %\addtolength{\rightskip}{-8.5cm}
     \includegraphics[width=\textwidth]{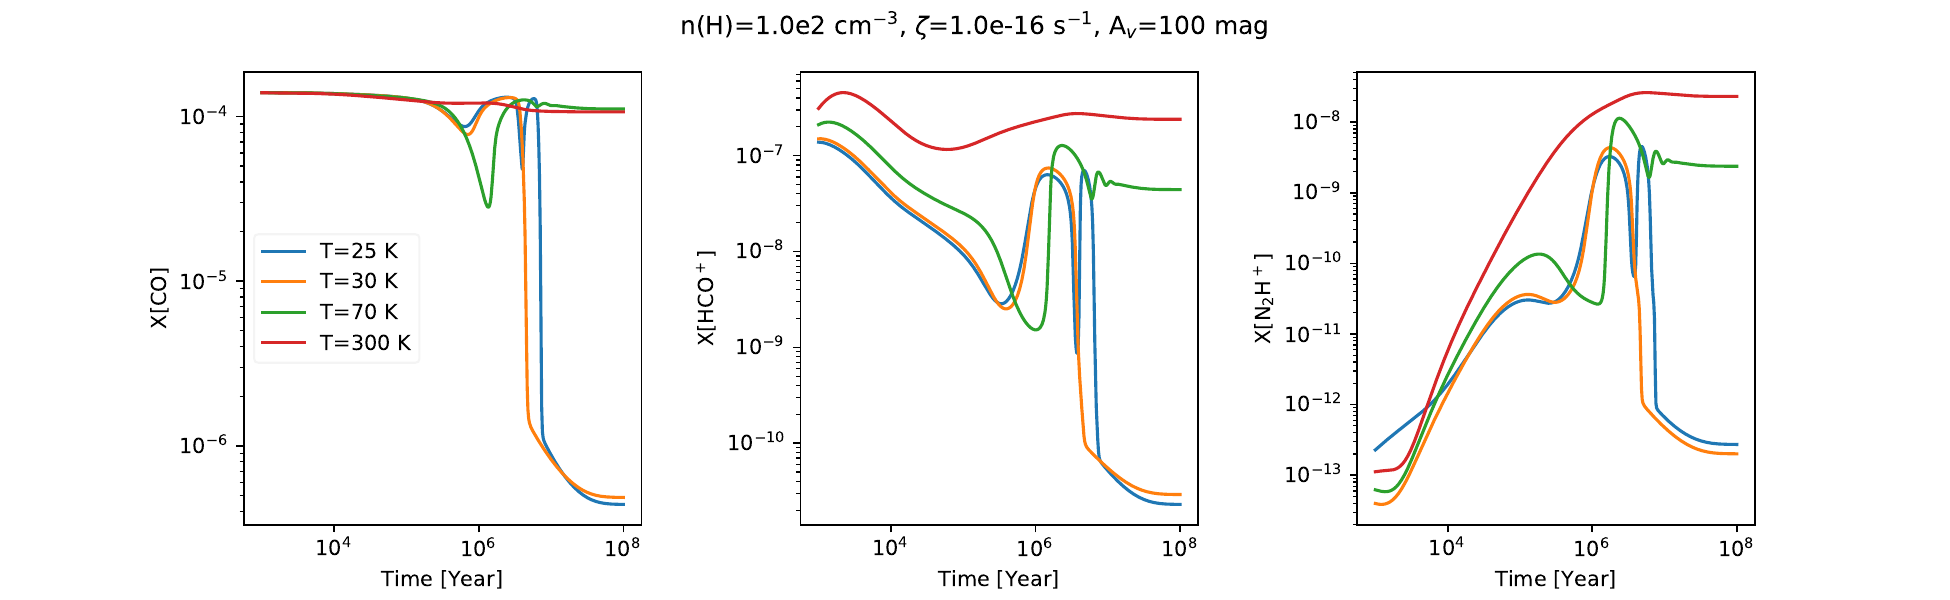}
     %\vspace{0.01cm}
     \caption{\tiny Influence of the temperature on the appearance of the vacillatory evolution of the species}
     \label{fig:os_T}
 \end{figure*}
%%%%%%%%%%%%%%%%%%%%%%%%%%%%%%%%%%%%%%%%%%%%%%%%%%5

\end{appendices}
