# Supplementary material for: Astrochemical modelling of infrared dark clouds
Source: arXiv:2111.05379 source file (2022-03-23)
Supplement: Supplementary file 4 [file appendix6.tex]

\begin{appendices}
%%%%%%%%%%%%%%%%%%%%%%%%%%%%%%%%%%%%%%%%%%%%%%%%%%%%%%%
\begin{figure*}[!ht]
   \centering
     %\addtolength{\leftskip} {-8cm}
    %\addtolength{\rightskip}{-8.5cm}
     \includegraphics[width=\textwidth]{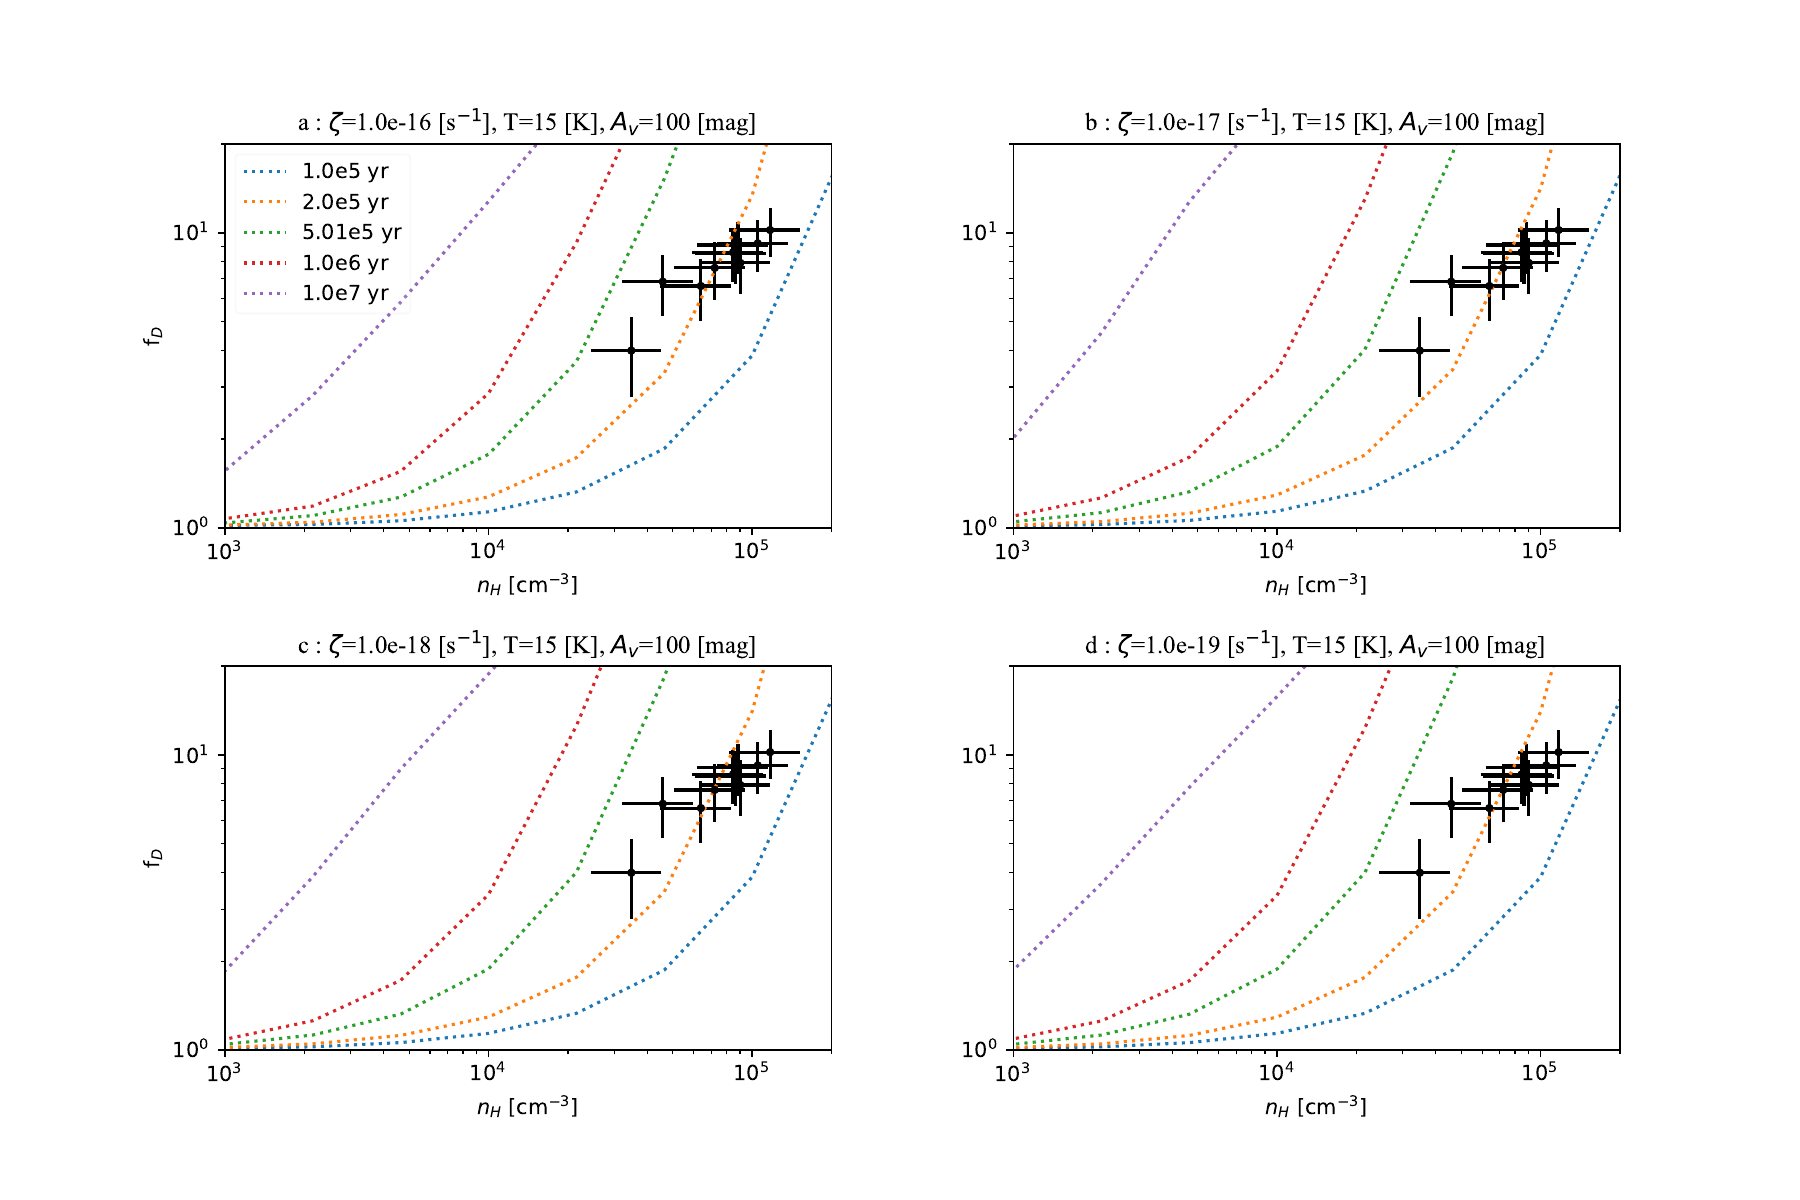}
     %\vspace{0.01cm}
     \caption{\tiny Observed CO depletion factor ($f_D$ versus estimated density compared with theoretical $f_D$, in the models with different $\zeta$.}
     \label{fig:fd_n_CRIR}
 \end{figure*}
 %%%%%%%%%%%%%%%%%%%%%%%%%%%%%%%%%%%%%%%%%%%%%
 \begin{figure*}[!ht]
   \centering
     %\addtolength{\leftskip} {-8cm}
    %\addtolength{\rightskip}{-8.5cm}
     \includegraphics[width=\textwidth]{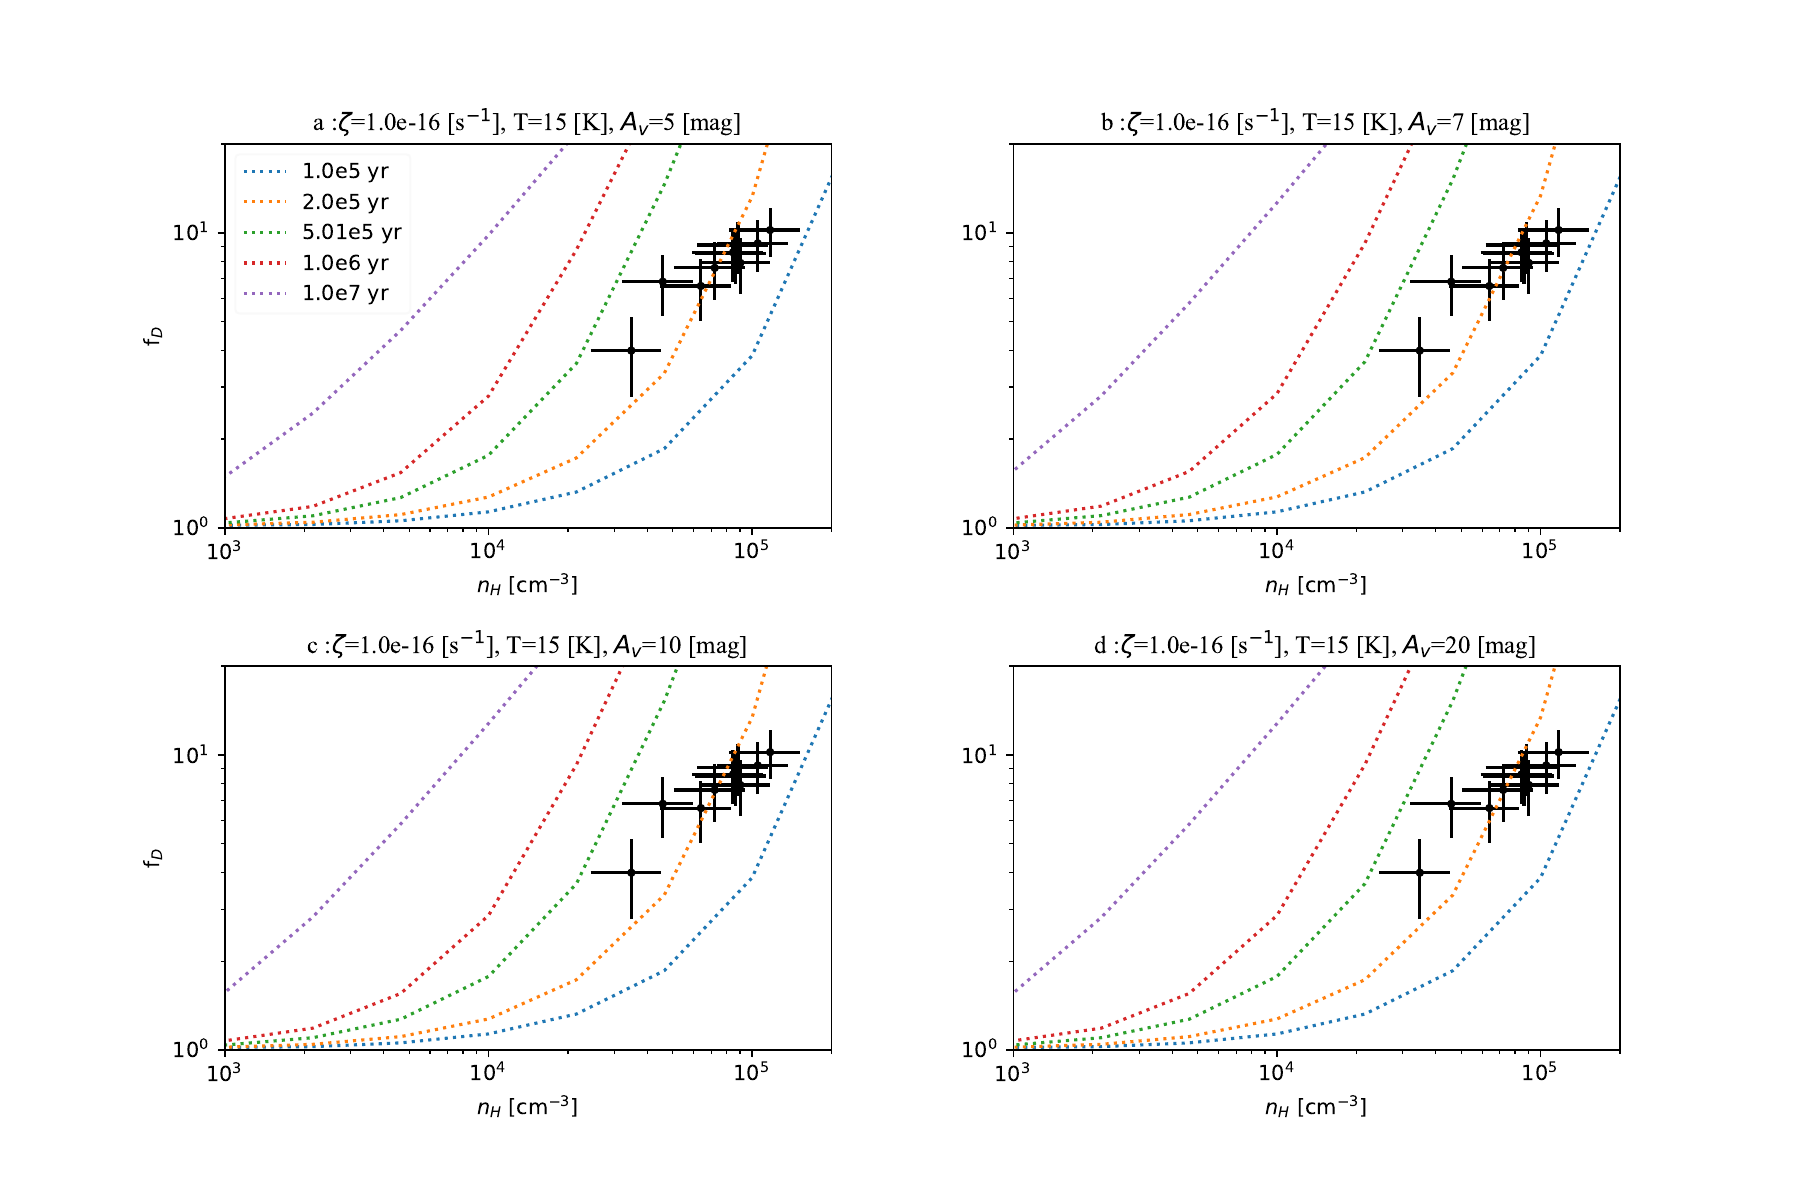}
     %\vspace{0.01cm}
     \caption{\tiny Observed CO depletion factor ($f_D$ versus estimated density compared with theoretical $f_D$, in the models with different $A_v$.}
     \label{fig:fd_n_av}
 \end{figure*}
 %%%%%%%%%%%%%%%%%%%%%%%%%%%%%%%%%%%%%%%%%%%%%%%%
  \begin{figure*}[!ht]
   \centering
     %\addtolength{\leftskip} {-8cm}
    %\addtolength{\rightskip}{-8.5cm}
     \includegraphics[width=\textwidth]{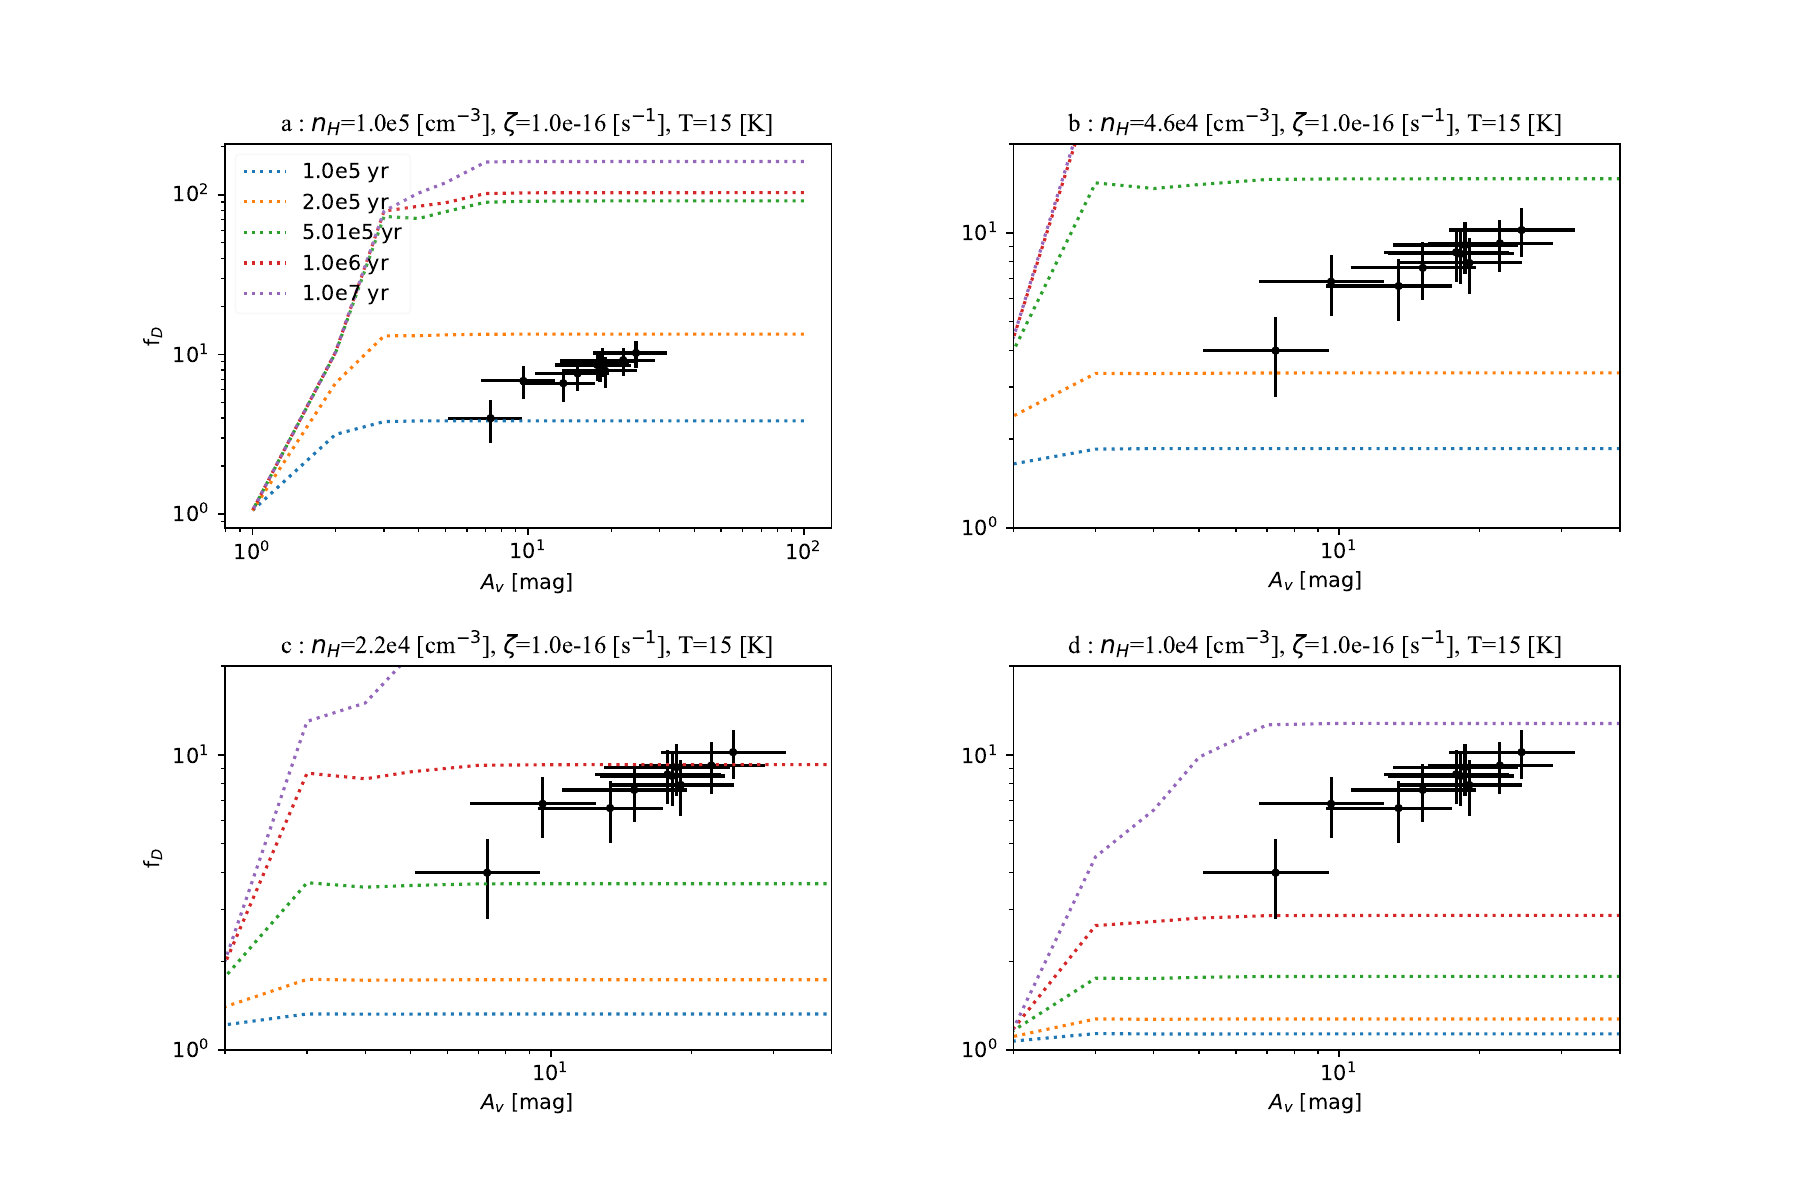}
     %\vspace{0.01cm}
     \caption{\tiny Observed CO depletion factor ($f_D$ versus estimated $A_v$ compared with theoretical $f_D$, in the models with different $n_H$.}
     \label{fig:fd_av_n}
 \end{figure*}
 %%%%%%%%%%%%%%%%%%%%%%%%%%%%%%%%%%%%%%%%%%%%%%%%

 \end{appendices}
