# Supplementary material for: Astrochemical modelling of infrared dark clouds
Source: arXiv:2111.05379 source file (2022-03-23)
Supplement: Supplementary file 5 [file appendix_tab.tex]

\begin{appendices}

%\begin{landscape}
\setlength{\tabcolsep}{8pt} % horizontal space
 % vertical space

\Large
\begin{table*}[htpb!]\centering
 \begin{adjustbox}{width=\textwidth}
  \begin{tabular}{c c c c c}
  \hline
  \hline
  & & XR & UR & R\\
  \hline
 P1 & main & 1.0e-18/1.70e5/1.0e5/15/20/0.107 & 1.0e-18/1.70e5/1.0e5/15/50/0.107 & 1.0e-19/2.00e7/2.2e4/20/5/0.070 \\
  & all & 1.0e-13/9.33e3/1.0e5/15/20/43.015 & 1.0e-18/1.00e8/2.2e5/20/10/37.754 & 4.6e-18/1.00e8/1.0e6/30/50/8.555\\
  \hline
  P2 & main & 2.2e-18/2.00e5/1.0e5/15/20/0.692 & 1.0e18/4.17e5/4.6e4/15/50/0.173 & 2.2e-19/2.24e6/1.0e4/15/5/0.020\\
 & all & 1.0e-13/2.88e3/1.0e5/15/20/52.752 & 1.0e-16/1.45e5/2.2e5/10/10/42.640 & 1.0e-17/5.62e7/1.0e6/30/50/16.256\\
  \hline
P3 & main & 2.2e-18/1.95e5/1.0e5/15/20/0.970 & 1.0e-18/3.98e5/4.6e4/15/10/0.494 & 2.2e-19/2.09e6/1.0e4/15/5/0.166\\
 & all & 1.0e-13/9.33e3/1.0e5/15/20/55.295 & 2.2e-18/5.25e7/2.2e5/20/10/47.706 & 4.6e-18/1.00e8/1.0e6/30/50/18.559\\
  \hline
  P4 & main & 2.2e-18/1.91e5/1.0e5/15/20/0.858 & 1.0e-18/3.89e5/4.6e4/15/10/0.312 & 2.2e-19/2.00e6/1.0e4/15/5/0.027\\
 & all & 1.0e-13/7.24e3/1.0e5/15/20/50.513 & 2.2e-18/5.13e7/2.2e5/20/10/43.412 & 4.6e-18/1.00e8/1.0e6/30/50/15.679\\
  \hline
  P5 & main & 2.2e-18/1.74e5/1.0e5/15/20/0.483 & 1.0e-18/3.55e5/4.6e4/15/10/0.208 & 4.6e-19/7.59e5/2.2e4/15/5/0.125\\
 & all & 1.0e-13/9.33e3/1.0e5/15/20/46.611 & 2.2e-18/5.13e7/2.2e5/20/10/43.081 & 4.6e-18/1.00e8/1.0e6/30/50/12.579\\
  \hline
  P6 & main & 4.6e-18/2.88e5/4.6e4/15/7/2.474 & 1.0e-18/7.24e5/2.2e4/15/5/1.730 & 4.6e-19/1.66e6/1.0e4/15/5/1.334\\
 & all & 4.6e-14/6.17e3/4.6e4/15/7/34.657 & 4.6e-19/1.48e7/2.2e4/20/5/13.309 & 4.6e-19/1.48e7/2.2e4/20/5/13.309\\
  \hline
  P7 & main & 1.0e-18/3.31e5/4.6e4/15/10/0.723 & 2.2e-19/8.32e5/2.2e4/15/20/0.392 & 1.0e-19/2.00e6/1.0e4/15/7/0.211 \\
 & all & 4.6e-14/2.45e4/4.6e4/15/10/40.362 & 1.0e-18/1.00e8/1.0e5/20/7/39.321 & 4.6e-18/1.00e8/1.0e6/30/50/11.610 \\
  \hline
  P8 & main & 4.6e-19/3.80e5/4.6e4/15/10/0.434 & 2.2e-19/8.13e5/2.2e4/15/7/0.271 & 1.0e-19/1.95e6/1.0e4/15/5/0.041\\
 & all & 4.6e-14/2.45e4/4.6e4/15/10/39.054 & 1.0e-19/7.76e6/2.2e4/15/7/37.034 & 4.6e-18/1.00e8/1.0e6/30/50/12.060 \\
  \hline
  P9 & main & 2.2e-18/1.78e5/1.0e5/15/20/0.483 & 1.0e-18/3.63e5/4.6e4/15/10/0.271 & 1.0e-19/2.34e6/1.0e4/15/100/0.117\\
 & all & 1.0e-13/9.33e3/1.0e5/15/20/49.929 & 2.2e-18/5.13e7/2.2e5/20/10/44.473 & 4.6e-18/1.00e8/1.0e6/30/50/13.954\\
  \hline
  P10 & main & 2.2e-18/3.16e5/4.6e4/15/10/0.507 & 4.6e-19/7.94e5/2.2e4/15/20/0.200 & 2.2e-19/1.91e6/1.0e4/15/100/0.055\\
 & all & 4.6e-14/1.00e3/4.6e4/15/10/44.001 & 2.2e-17/5.01e5/4.6e4/10/7/38.312 & 4.6e-18/1.00e8/1.0e6/30/50/14.364\\

        \hline
        \hline
    \end{tabular}
  \end{adjustbox}
  \vspace*{1mm}
  \caption{Extracted Astrochemical parameters of the best models by applying observed abundances in Restricted (R), Ultra restricted (UR) and Extra restricted (XR) regions, using main species, [CO],[HCO$^+$] and [N$_2$H$^+$] (A) and all observed abundances (B). The extracted parameters are $\zeta$ [s$^{-1}$], Time [year], $\mathrm{n}_H$ [cm$^{-3}$], T [K], $\mathrm{A}_v$ [mag] and $\chi^2$, respectively from left to right.}
  \label{tab:gen_table}
  
\end{table*}
%\end{landscape}

\end{appendices}
